# Supplementary material for: Algebraic fibre spaces with strictly nef relative anti-log canonical divisor
Source: arXiv:2111.05234 source file (2021-11-09)
Supplement: Supplementary file 1 [file appendix.tex]

\appendix
\titleformat{\section}{\Large\bfseries}{Appendix \thesection}{1em}{}
%\addcontentsline{toc}{section}{Appendix~A\quad Proof of Serrano's conjecture for Gorenstein terminal threefolds}

\addappheadtotoc

%\begin{appendices}

\section{Proof of Serrano's conjecture for  mildly singular non-Calabi-Yau threefolds}
\label{appendix}
In this appendix, we study  {\hyperref[main-conj-singular-arbitrary]{Question  \ref*{main-conj-singular-arbitrary}}}. 
Our main result is {\hyperref[main_theorem_Goren_ter_3fold]{Theorem   \ref*{main_theorem_Goren_ter_3fold}}} below, which generalizes \cite[Theorem 0.4]{CCP08} (cf.~\cite[Section 4]{Ser95}) to the singular threefold case.

\begin{thm}\label{main_theorem_Goren_ter_3fold}
Let $X$ be a normal projective threefold with only klt singularities, 
and $L_X$ a strictly nef divisor on $X$.
Suppose one of the following holds.
\begin{enumerate}
\item[(1)] The Kodaira dimension $\kappa(X)\geqslant 1$;
\item[(2)] The augmented irregularity $q^{\circ}(X)>0$, and either $X$ is $\mathbb{Q}$-factorial or $X$ has only canonical singularities; or
\item[(3)] $X$ is uniruled, and  has only isolated $\mathbb{Q}$-factorial Gorenstein canonical singularities. 
\end{enumerate}
Then $K_X+tL_X$ is ample for sufficiently large $t\gg 1$.
\end{thm}

In (3), the condition on singularities is  to avoid flips when we run the minimal model program (MMP for short); see  {\hyperref[lem_del14]{Lemma  \ref*{lem_del14}}}, {\hyperref[lem_canonical_terminal]{Lemma  \ref*{lem_canonical_terminal}}}, and {\hyperref[rem_composition_conic]{Remark  \ref*{rem_composition_conic}}}.

Terminal threefolds having isolated singularities, we have the following corollary immediately.

\begin{cor}\label{main_Goren_ter_3fold}
Let $X$ be a $\mathbb{Q}$-factorial Gorestein terminal projective threefold, and $L_X$ a strictly nef $\mathbb{Q}$-divisor on $X$.
Suppose that either $\kappa(X)\neq 0$ or $q^{\circ}(X)\neq 0$.
Then $K_X+tL_X$ is ample for sufficiently large $t\gg 1$.
\end{cor}

In {\hyperref[main-conj-singular-arbitrary]{Question  \ref*{main-conj-singular-arbitrary}}},	if $\kappa(X)=0$,  then things will become quite different and more harder.
In this case, one can start from  $K_X\equiv 0$ (cf.~{\hyperref[prop-q-effective]{Proposition  \ref*{prop-q-effective}}}) and then
{\hyperref[main-conj-singular-arbitrary]{Question  \ref*{main-conj-singular-arbitrary}}} predicts that strict nefness is equivalent to ampleness, which relates to the abundance conjecture.
 We refer to \cite{LS20} for a recent progress from this direction.

The remaining part of the appendix is devoted to the proof of {\hyperref[main_theorem_Goren_ter_3fold]{Theorem   \ref*{main_theorem_Goren_ter_3fold}}}. 
For the proof, we follow the ideas in \cite{CCP08}, though in our situation, the appearance of singularities will make things more complicated. 
{\hyperref[main_theorem_Goren_ter_3fold]{Theorem   \ref*{main_theorem_Goren_ter_3fold}}} is obtained as the union of {\hyperref[kappa>=1]{Theorem   \ref*{kappa>=1}}}   (cf.~{\hyperref[thm_higher-dim-kappa>=1]{Proposition   \ref*{thm_higher-dim-kappa>=1}}}),
{\hyperref[coro_q0>0]{Corollary   \ref*{coro_q0>0}}}, {\hyperref[remark_conclude_excep_tocurve]{Remark   \ref*{remark_conclude_excep_tocurve}}}  and {\hyperref[thm_3fold_surface_curve]{Theorem    \ref*{thm_3fold_surface_curve}}}.
%Moreover, without causing any confusion, we provide  in higher dimensions for readers' comparison. 

Now, we begin our proof of {\hyperref[main_theorem_Goren_ter_3fold]{Theorem   \ref*{main_theorem_Goren_ter_3fold}}}.
First, we prove a more general (pair) version of {\hyperref[main_theorem_Goren_ter_3fold]{Theorem   \ref*{main_theorem_Goren_ter_3fold} (1)}}.

\begin{thm}[{cf.~{\hyperref[main_theorem_Goren_ter_3fold]{Theorem   \ref*{main_theorem_Goren_ter_3fold} (1)}}}]\label{kappa>=1}
Let $(X,\Delta)$ be a projective klt threefold pair, and $L_X$ a strictly nef $\mathbb{Q}$-Cartier divisor on $X$.
Suppose that the Iitaka dimension  $\kappa(X,K_X+\Delta)\geqslant 1$.
Then $K_X+\Delta+tL_X$ is ample for sufficiently large $t$.
\end{thm}

\begin{proof}
Since $L_X$ is strictly nef, by 	{\hyperref[lem_strict_nef_k]{Lemma \ref*{lem_strict_nef_k}}}, $K_X+\Delta+tL_X$ is strictly nef for $t\gg 1$.
Clearly, $K_X+\Delta$ is pseudo-effective.
Hence, it follows from \cite[Corollary D]{LP20A} that $K_X+\Delta+tL_X$ is numerically equivalent to a semiample $\mathbb{Q}$-divisor $M$.
Then with $M$ replaced by a multiple, it defines a morphism $\sigma:X\to Y$ with $M=\sigma^*\mathcal{O}_Y(1)$.
Therefore, the strict nefness of $M$ together with the projection formula implies that $\sigma$ is a finite morphism and thus $M$ is  ample.
So our theorem is proved.
\end{proof}

As a higher dimensional analogue of {\hyperref[kappa>=1]{Theorem  \ref*{kappa>=1}}},
we show the following proposition by further requiring  the pair $(X,\Delta)$ having only canonical singularities.
Note that, this is also an extension of \cite[Theorem 2.6]{CCP08} and has its independent interests.
%We refer readers to \cite[Sections 2 and 3]{CCP08} for the smooth threefold case. 
\begin{prop}[{cf.~{\hyperref[kappa>=1]{Theorem  \ref*{kappa>=1}}} and \cite[Theorem 2.6]{CCP08}}]\label{thm_higher-dim-kappa>=1}
Let $(X,\Delta)$ be a projective canonical pair, and $L_X$ a strictly nef $\mathbb{Q}$-divisor on $X$.
Suppose  the Iitaka dimension $\kappa(a(K_X+\Delta)+bL_X)\geqslant\dim X-2$ for some $a,b\geqslant 0$.
Then $(K_X+\Delta)+tL_X$ is ample for sufficiently large $t$.
\end{prop}

\begin{proof}
If $\dim X\leqslant 2$, then our theorem follows from {\hyperref[main_thm_surface]{Proposition \ref*{main_thm_surface}}}.
So we may assume $\dim X-2\geqslant 1$.
By {\hyperref[lem_strict_nef_k]{Lemma  \ref*{lem_strict_nef_k}}}, $K_X+\Delta+tL_X$ is strictly nef for $t\gg 1$. 
With $b$ replaced by $b/a$ (if $a\neq 0$), we may further assume  $0\leqslant a\leqslant 1$.
Let $\pi:X\dashrightarrow Y$ be the Iitaka fibration of $a(K_X+\Delta)+bL_X$ (with $\dim Y\geqslant 1$).
Resolving the indeterminacy of $\pi$ and the singularities of $X$, we get the induced morphisms $\pi_1:\widetilde{X}\to X$ and $\pi_2:\widetilde{X}\to Y$ such that  $\widetilde{X}$ is smooth and
\begin{equation}\label{equ_1}
	K_{\widetilde{X}}+\widetilde{\Delta}=\pi_1^*(K_X+\Delta)+\sum a_iE_i
\end{equation}
with $\widetilde{\Delta}:=(\pi_1)_*^{-1}\Delta$ and $a_i\geqslant 0$, noting that $(X,\Delta)$ is a projective canonical pair.
Moreover, there exists an ample $\mathbb{Q}$-divisor $H$ on $Y$ such that
\begin{equation}\label{equ_2}
\pi_1^*(a(K_X+\Delta)+bL_X)\sim_{\mathbb{Q}}\pi_2^*H+E_0.	
\end{equation}
Here, some multiple $nE_0$ is the fixed component of $|n\pi_1^*(a(K_X+\Delta)+bL_X)|$ (which defines $\pi_2$) and hence $E_0\ge 0$. 
Let $L_{\widetilde{X}}:=\pi_1^*L_X$, being almost strictly nef (cf.~{\hyperref[defn-almost-sn]{Definition \ref*{defn-almost-sn}}}) 
%(cf.~{\hyperref[sec_pre]{Section \ref*{sec_pre}}}) 
on $\widetilde{X}$.
Then for a general fibre $F$ of $\pi_2$, the restriction $L_{\widetilde{X}}|_F$ is almost strictly nef.

If $\kappa(a(K_X+\Delta)+bL_X)=\dim X$, then our theorem follows from {\hyperref[lem-big-ample]{Lemma  \ref*{lem-big-ample}}}.
If $\kappa(a(K_X+\Delta)+bL_X)=\dim X-1$, then  $L_{\widetilde{X}}|_F$ is clearly ample.
If $\kappa(a(K_X+\Delta)+bL_X)=\dim X-2$, then $\dim F=2$; in this case, it follows from \cite[Theorem 26]{Cha20} that $K_F+tL_{\widetilde{X}}|_F$ is big for $t\gg 1$ and hence $(K_{\widetilde{X}}+\widetilde{\Delta}+tL_{\widetilde{X}})|_{F}$ is big for $t\gg 1$.
Let us fix the ample $\mathbb{Q}$-divisor $H$ on $Y$ in {\hyperref[equ_2]{Equation  (\ref*{equ_2})}}.

In each case, we see that 
$K_{\widetilde{X}}+\widetilde{\Delta}+tL_{\widetilde{X}}+\pi_2^*H$
is big for $t\gg 1$: fixing one $t$ such that $(K_{\widetilde{X}}+\widetilde{\Delta}+tL_{\widetilde{X}})|_{F}$ is big, we see that  $A_k:=(K_{\widetilde{X}}+\widetilde{\Delta}+tL_{\widetilde{X}})+k\pi_2^*H$ is big for $k\gg 1$ (cf.~e.g. \cite[Lemma 3.23]{KM98}).
Since $K_{\widetilde{X}}+\widetilde{\Delta}+tL_{\widetilde{X}}=\pi_1^*(K_X+\Delta+tL_X)+\sum a_iE_i$ is   pseudo-effective, our $A_1=K_{\widetilde{X}}+\widetilde{\Delta}+tL_{\widetilde{X}}+\pi_2^*H=\frac{1}{k}(A_k+(k-1)(K_{\widetilde{X}}+\widetilde{\Delta}+tL_{\widetilde{X}}))$ is big.

%By \cite[Lemma 2.60]{KM98}, there exist an ample $\mathbb{Q}$-divisor $G$ and an effective $\mathbb{Q}$-divisor $M\ge 0$ on $\widetilde{X}$ such that
%$A_1\equiv G+M\ge G$.
Set $N:=(1-a)(K_{\widetilde{X}}+\widetilde{\Delta})+(t-b)L_{\widetilde{X}}$, which is pseudo-effective for $t\gg 1$ (cf.~{\hyperref[lem_strict_nef_k]{Lemma  \ref*{lem_strict_nef_k}}} and {\hyperref[equ_1]{Equation  (\ref*{equ_1})}}.
Following from {\hyperref[equ_1]{Equation  (\ref*{equ_1})}} and {\hyperref[equ_2]{Equation  (\ref*{equ_2})}}, we have
\begin{align*}
2(K_{\widetilde{X}}+\widetilde{\Delta}+tL_{\widetilde{X}})&=A_1+(a(K_{\widetilde{X}}+\widetilde{\Delta})+bL_{\widetilde{X}}-\pi_2^*H)+N\\
&=
A_1+\pi_1^*(a(K_X+\Delta)+bL_X)+\sum aa_iE_i-\pi_2^*H+N\\
&\sim_{\mathbb{Q}} A_1+E_0+\sum aa_iE_i+N(\ge A_1+N),
\end{align*}
which is big for $t\gg 1$.
Thus, the push-forward $K_X+\Delta+tL_X$ is also big for $t\gg1$ (cf.~\cite[Lemma 4.10(i\!i\!i) and its proof]{FKL16}).
So our theorem follows from {\hyperref[lem-big-ample]{Lemma  \ref*{lem-big-ample}}}.
\end{proof}

With  the same proof of \cite[Theorem 3.1]{CCP08}  after replacing \cite[Theorem 0.3, Lemma 1.5, Propositions 1.7, 1.8]{CCP08} by 
{\hyperref[mainthm-RC]{Theorem \ref*{mainthm-RC}}}, {\hyperref[lem-big-ample]{Lemma  \ref*{lem-big-ample}}},  {\hyperref[prop_Q-Goren_surface]{Proposition  \ref*{prop_Q-Goren_surface}}} and {\hyperref[prop-q-effective]{Proposition  \ref*{prop-q-effective}}}, respectively, we  get the theorem below.   
For readers' convenience, we  include a detailed proof here. 
\begin{thm}[{cf.~\cite[Theorem 3.1]{CCP08}, \cite[Theorem 8.1]{LP20B}}]\label{thm_alb}
Let $(X,\Delta)$ be a   projective klt threefold pair, and $L_X$ a  strictly nef $\mathbb{Q}$-divisor on $X$.
Suppose there exists a non-constant morphism $\pi:X\to A$ to an abelian variety (this is the case when $q(X)>0$).
Then $K_X+\Delta+tL_X$ is numerically equivalent to a non-zero effective divisor for  some $t\gg 1$. 
If $X$ is further assumed to be either $\mathbb{Q}$-factorial, or have only canonical singularities, 
then $K_X+tL_X$ is ample for $t\gg 1$.
\end{thm}

\begin{proof}
Replacing $L_X$ by a multiple, we may assume that $L_X$ is Cartier.
Let $m$ be the Cartier index of $K_X+\Delta$, $D_t:=2m(K_X+\Delta+tL_X)$ and $\mathcal{F}_t:=\pi_*\mathcal{O}_X(D_t)$. 
Fix one $t>6m$ such that $D_t$ is strictly nef and  $D_t|_{F}$ is ample for a general fibre $F$ of $\pi$ (cf.~{\hyperref[main_thm_surface]{Proposition \ref*{main_thm_surface}}} and \cite[Theorem 1.37]{KM98}). 
%With $m$ replaced by a multiple, we may further assume that $D_t|_{F_0}$ is very ample for some fibre $F_0$ and thus $\mathcal{F}_t$ is a non-zero sheaf, noting that $\pi^*\mathcal{F}_t\to \mathcal{O}_X(D_t)$ is surjective around $F_0$.
%Since $D_t$ is $\pi$-ample over a general point of $\pi(X)$, 
Then it is easy to verify that $D_t$ is $\pi$-big  (cf.~\cite[Definition 3.22]{KM98}). 
Since $D_t-(K_X+\Delta)=(2m-1)(K_X+\Delta+tL_X)+tL_X$ is  $\pi$-big and $\pi$-nef, by the relative base-point-free theorem (cf.~\cite[Theorem 3.24]{KM98}), $nD_t$ is $\pi$-free  for all $n\gg 1$.
Hence, with $m$ replaced by a multiple, we may further assume that $D_t$ is $\pi$-free (i.e., $\pi^*\mathcal{F}_t\to \mathcal{O}_X(D_t)$ is surjective), and thus $\mathcal{F}_t$ is a non-zero sheaf.

Let $\hat{A}=\textup{Pic}^0(A)$ be the dual abelian variety and $\mathcal{P}$  the normalized Poincar\'e line bundle (in the sense that both $\mathcal{P}|_{A\times\{\hat{0}\}}$ and $\mathcal{P}|_{\{0\}\times\hat{A}}$ are trivial).
Denote by $p_A$ and $p_{\hat{A}}$ the projections of $A\times\hat{A}$ onto $A$ and $\hat{A}$.
For any ample line bundle $\hat{M}$ on $\hat{A}$, we define the isogeny $\phi_{\hat{M}}:\hat{A}\to A$  by $\phi_{\hat{M}}(\hat{a})=t_{\hat{a}}^*\hat{M}^{\vee}\otimes\hat{M}$, and
let $M:=(p_{A})_*(p_{\hat{A}}^*\hat{M}\otimes\mathcal{P})$ be the vector bundle on $A$.
Recall that $\phi_{\hat{M}}^*(M^{\vee})\simeq\hat{M}^{\oplus\dimcoh^0(\hat{M})}$ (cf.~\cite[Proposition 3.11 (1)]{Muk81}). 
%Then one has that $\phi_{\hat{M}}^*(M^{\vee})\cong\oplus_{h^0(\hat{M})}\hat{M}$  
\begin{claim}\label{claim_fm}
$H^i(A,\mathcal{F}_t\otimes M^{\vee})=0$ for any  $t\gg1$ and any ample line bundle $\hat{M}$ on $\hat{A}$. 
\end{claim}
Suppose the claim for the time being.
Then it follows from \cite[Theorem 1.2 and Corollary 3.2]{Hac04} that
we have a chain of inclusions
$V^0(\mathcal{F}_t)\supseteq V^1(\mathcal{F}_t)\supseteq\cdots\supseteq V^n(\mathcal{F}_t)$, 
where $V^i(\mathcal{F}_t):=\{P\in\textup{Pic}^0(A)~|~\dimcoh^i(A,\mathcal{F}_t\otimes P)\neq 0\}$.
%denotes the locus where the $i$-th cohomology does not vanish.
Recall that $\mathcal{F}_t$ is a  non-zero sheaf by the choice of our $m$. 
If  $V^i(\mathcal{F}_t)=\emptyset$ for all $i$, then the Fourier-Mukai transform of $\mathcal{F}_t$ is zero, noting that $\mathcal{P}|_{A\times\{P\}}\cong P$ and 
$\RDer^i\!(p_{\hat{A}})_*(p_A^*\mathcal{F}_t\otimes\mathcal{P})_P=\Coh^i(A,\mathcal{F}_t\otimes P)$ 
for any $P\in\textup{Pic}^0(X)$.  
By \cite[Theorem 2.2]{Muk81},  $\mathcal{F}_t$ is a zero sheaf, which is absurd. 
So $V^0(\mathcal{F}_t)\neq\emptyset$ and thus
$\dimcoh^0(X,D_t+\pi^*P)\neq 0$ for some $P\in\textup{Pic}^0(A)$.
If $D_t+\pi^*P\sim 0$, then $-(K_X+\Delta)$ is strictly nef; hence $X$ is rationally connected and  $q(X)=0$ by {\hyperref[mainthm-RC]{Theorem \ref*{mainthm-RC}}},  which contradicts the existence of $\pi$. 
So  $D_t\equiv D_t+\pi^*P\sim E$ for some non-zero effective divisor $E$, 
%Let $L_X':=L_X+\frac{1}{2mt}\pi^*P\equiv L_X$ be a shifted $\mathbb{Q}$-divisor.
%Then $2m(K_X+tL_X')=D_t+\pi^*P\sim E$, 
and the first part of our theorem is proved.

If $X$ is further assumed to be  $\mathbb{Q}$-factorial (resp. have only canonical singularities), then we apply the first part of our theorem for the klt (resp. canonical) pair $(X,0)$, and thus $K_X+tL_X$ is numerically equivalent to a non-zero effective divisor; hence, the second part of our theorem 
 follows from {\hyperref[prop-q-effective]{Proposition  \ref*{prop-q-effective}}} (resp. {\hyperref[prop-klt-eff-ample]{Proposition  \ref*{prop-klt-eff-ample}}}). 
 
\par \vskip 1pc \noindent
\textbf{Proof of {\hyperref[claim_fm]{Claim \ref*{claim_fm}}}.}
Fix an ample divisor $H$ on $A$. 
Since $D_{t}$ is  $\pi$-big, our $D_t+\pi^*H$ is big, noting that $D_t$ is not only $\pi$-big, but also nef (and hence pseudo-effective) (cf.~\cite[Lemma 3.23]{KM98}).
Therefore, $D_t+\pi^*(H+P)$ is nef and big for any $P\in\textup{Pic}^0(A)$. 
Since $(X,\Delta)$ has at worst klt singularities and 
%Set 
%$$\widetilde{D}_0:=2m(K_X+tL_X)+g^*H=D_t+g^*H.$$
%Then $\widetilde{D}_0-K_X=\frac{2m-1}{2m}D_t+tL_X+g^*H$ is again nef and big.
%By the base-point-free theorem, $k\widetilde{D}_0$ is globally generated for some $k\gg 1$. 
%Taking $D$ to be a general smooth member in $|k\widetilde{D}_0|$,  we see that
$$D_t+\pi^*(H+P)=K_X+\Delta+\frac{2m-1}{2m}(D_t+\pi^*(H+P))+\frac{1}{2m}\pi^*(H+P)+tL_X=:K_X+\Delta+\widetilde{D}$$
 %and , $(X,\frac{2m-1}{2mk}D)$ is klt.
with $\widetilde{D}$ being a nef and big $\mathbb{Q}$-Cartier Weil divisor, it follows from  Kawamata-Viehweg Vanishing Theorem (cf. e.g. \cite[Theorem 2.70]{KM98}) that 
$$\Coh^j(A,\mathcal{F}_t\otimes H\otimes P)\simeq\Coh^j(X,D_t+\pi^*H+\pi^*P)\simeq0$$
for all $j\geqslant 1$ (recall that $\mathcal{F}_t:=\pi_*\scrO_X(D_t)$). 
The first equality is due to $\RDer^j\pi_*(D_t+\pi^*H+\pi^*P)=0$ for all $j\geqslant 1$ (cf.~\cite[Remark 1-2-6]{KMM87}).
%Applying Kawamata-Viehweg Vanishing Theorem and \cite[Theorem 1-2-5]{KMM87} again to $D_t+\pi^*H+\pi^*P$ with $P\in\textup{Pic}^0(A)$, we have
%$$H^j(A,\mathcal{F}_t\otimes H\otimes P)=H^j(X,D_t+\pi^*H+\pi^*P)=0$$
%for all $j\ge 1$.
Following the same terminology as in \cite[Definition 2.3]{Muk81}, for any ample line bundle $H$ on $A$, we say that \textit{the index theorem of degree zero holds for the sheaf $\mathcal{F}_t\otimes H$} (which is also abbreviated to ``$IT^0$'' in \cite[Proof of Theorem 3.1]{CCP08}).

Let $\hat{M}$ be any ample line bundle on $\hat{A}$, and $\phi_{\hat{M}}:\hat{A}\to A$  the isogeny defined  in the beginning of the proof. 
Let $\hat{\pi}:\hat{X}:=X\times_A\hat{A}\to \hat{A}$ be the base change with the induced map $\varphi:\hat{X}\to X$ being \'etale.
Then we have $K_{\hat{X}}=\varphi^*K_X$ and $L_{\hat{X}}:=\varphi^*L_X$ is strictly nef on $\hat{X}$.
Let $\mathcal{G}_t:=\hat{\pi}_*\varphi^*D_t$.
With the same argument as above, we see that, for any ample line bundle $\hat{M}$ on $\hat{A}$, the index theorem of degree zero holds for the sheaf $\mathcal{G}_t\otimes\hat{M}$. 
Since $\phi_{\hat{M}}$ is flat and $\pi$ is projective, we have
\begin{align*}
&~\phi_{\hat{M}}^*(\mathcal{F}_t\otimes M^{\vee})=\phi_{\hat{M}}^*(\pi_*D_t\otimes M^{\vee})=\phi_{\hat{M}}^*\pi_*(D_t\otimes \pi^*M^{\vee})=\hat{\pi}_*\varphi^*(D_t\otimes \pi^*M^{\vee})\\
&=\hat{\pi}_*(\varphi^*D_t\otimes\hat{\pi}^*\phi_{\hat{M}}^*M^{\vee})=\hat{\pi}_*(\varphi^*D_t\otimes\hat{\pi}^*(\oplus \hat{M}))=\oplus(\hat{\pi}_*\varphi^*D_t\otimes\hat{M})=\oplus(\mathcal{G}_t\otimes\hat{M}).
\end{align*}
Therefore, the index theorem of degree zero holds for the sheaf $\phi_{\hat{M}}^*(\mathcal{F}_t\otimes M^{\vee})$, i.e., for any $j\ge 1$ and $\hat{P}\in\textup{Pic}^0(\hat{A})=A$, 
we have the vanishing $H^j(\hat{A},\phi_{\hat{M}}^*(\mathcal{F}_t\otimes M^{\vee})\otimes\hat{P})=0$. 
Since $\phi_{\hat{M}}^*$ is finite, taking $\hat{P}:=\mathcal{O}_{\hat{A}}$, we see that $H^j(A,\mathcal{F}_t\otimes M^{\vee}\otimes (\phi_{\hat{M}})_*\mathcal{O}_{\hat{A}})=0$.
Now that $\mathcal{O}_A$ is a direct summand of $(\phi_{\hat{M}})_*\mathcal{O}_{\hat{A}}$ (cf.~\cite[Proposition 5.7]{KM98}),  our claim is thus  proved.
\end{proof}

We give a few remarks on {\hyperref[thm_alb]{Theorem   \ref*{thm_alb}}}.
First,  when $K_X+\Delta$ is pseudo-effective, \cite[Theorem 8.1]{LP20B} shows a stronger version of {\hyperref[thm_alb]{Theorem   \ref*{thm_alb}}} in higher dimensions. 
However, our {\hyperref[thm_alb]{Theorem   \ref*{thm_alb}}} here relaxes this assumption by assuming the nef divisor $L_X$ being strictly nef. 
Second, we note that, the first part of  {\hyperref[thm_alb]{Theorem   \ref*{thm_alb}}} actually holds for $n$-dimensional $X$ if we assume that  {\hyperref[main-conj-singular-arbitrary]{Question  \ref*{main-conj-singular-arbitrary}}} has a positive answer for the case when $\dim X\leqslant n-1$.

As a consequence of {\hyperref[thm_alb]{Theorem   \ref*{thm_alb}}}, we have the corollary below. 
\begin{cor}[{cf.~{\hyperref[main_theorem_Goren_ter_3fold]{Theorem   \ref*{main_theorem_Goren_ter_3fold} (2)}}}]\label{coro_q0>0}
Let $X$ be a  normal projective threefold with at worst klt singularities, and $L_X$ a strictly nef $\mathbb{Q}$-divisor on $X$.
Suppose that the augmented irregularity $q^\circ(X)>0$.
Suppose further that either $X$ is $\mathbb{Q}$-factorial, or $X$ has only canonical singularities.
Then $K_X+tL_X$ is ample for sufficiently large $t$.
\end{cor}

\begin{proof}
Let $\pi:X'\to X$ be a quasi-\'etale cover such that $q(X')>0$, and $L_{X'}:=\pi^*L_X$.

First, we assume that $X$ has only canonical singularities. 
In this case, $X'$ also has only canonical singularities (cf.~\cite[Proposition 5.20]{KM98}).
By {\hyperref[thm_alb]{Theorem   \ref*{thm_alb}}}, our $K_{X'}+tL_{X'}$ and hence $K_X+tL_X$ are ample.

Second, we assume that $X$ is $\mathbb{Q}$-factorial.
In this case, applying \cite[Proposition 5.20]{KM98} again, our $X'$  has only klt singularities. 
Then, it follows from {\hyperref[thm_alb]{Theorem   \ref*{thm_alb}}} that our $K_{X'}+tL_{X'}\equiv E>0$ for some $t\gg 1$. 
So the push-down $\deg(\pi)\cdot(K_X+tL_X)$ is weakly numerically equivalent to $\pi_*(E)>0$ (cf.~\cite[Definition 2.2]{MZ18}). 
Since $X$ is $\mathbb{Q}$-factorial, weak numerical equivalence of divisors coincide with numerical equivalence (cf.~\cite[Lemma 3.2]{Zha16}); hence $K_X+tL_X\equiv \frac{1}{\deg(\pi)}\pi_*(E)$. 
By {\hyperref[prop-q-effective]{Proposition  \ref*{prop-q-effective}}}, our corollary follows.
\end{proof}

From {\hyperref[lem_del14]{Lemma  \ref*{lem_del14}}} to {\hyperref[remark_conclude_excep_tocurve]{Remark     \ref*{remark_conclude_excep_tocurve}}} below, 
we shall run the first step of the MMP for the proof of {\hyperref[main_theorem_Goren_ter_3fold]{Theorem   \ref*{main_theorem_Goren_ter_3fold} (3)}}.  
Recall that a \textit{contraction} of a  normal projective variety $X$ is a surjective morphism with connected fibres.
A contraction $\pi:X\to S$ is said to be \textit{elementary} if the relative Picard number $\rho(X/S)=1$.

The following lemma is a special  case of \cite[Theorem 2.2]{Del14},  which extends  \cite[Theorem 4]{Cut88} to the  isolated canonical singularities so as to avoid  small contractions.

\begin{lemme}[{cf.~\cite[Theorem 2.2]{Del14}}]\label{lem_del14}
Let $X$ be a $\mathbb{Q}$-factorial Gorenstein normal projective threefold with only isolated  canonical singularities. 
Let $\varphi:X\to Y$ be a birational $K_X$-negative contraction  of an extremal face $R$ whose fibres are at most one-dimensional.
%Suppose, moreover, that the exceptional locus of $\varphi$ is contained in the Gorenstein locus $G$ of $X$.
Then the following assertions hold.
\begin{enumerate}
\item[(1)] 
The exceptional locus $E:=\textup{Exc}(\varphi)$ is a disjoint union of prime divisors, 
$\varphi$ is a composition of divisorial contractions mapping exceptional divisors onto curves, and $Y$ has only isolated canonical singularities.
\item[(2)] There exists a finite subset $T\subseteq Y$  such that $Y\backslash T\subseteq Y_{\textup{reg}}$,  $\text{codim}~\varphi^{-1}(T)\ge 2$, $X\backslash \varphi^{-1}(T)\subseteq X_{\textup{reg}}$ and 
$$\varphi|_{X\backslash\varphi^{-1}(T)}:X\backslash \varphi^{-1}(T)\to Y\backslash T$$
is the simultaneous blow-up of   smooth curves.
In particular, $K_X=\varphi^*(K_Y)+\sum E_i$ with $E_i$ being exceptional, and $\textup{Sing}~(\sum E_i)\subseteq \varphi^{-1}(\textup{Sing}~\sum\varphi(E_i))$.
\item[(3)] Let $f\subseteq X$ be an irreducible curve such that $[f]\in R$. Then
$K_X\cdot f=E\cdot f=-1$.
\end{enumerate}
\end{lemme}

Based on {\hyperref[lem_del14]{Lemma  \ref*{lem_del14}}}, we establish the following lemma on an elementary contraction (of an extremal ray), which is a key to reduce the isolated canonical singularities to terminal singularities via the terminalization.

\begin{lemme}\label{lem_canonical_terminal}
Let $X$ be a normal projective threefold with only isolated $\mathbb{Q}$-factorial Gorenstein canonical singularities. 
Suppose that $\pi:X\to Y$ is a birational elementary  contraction of a $K_X$-negative extremal ray.
Then we have the following commutative diagram
\[\xymatrix{\widetilde{X}\ar[r]^{\widetilde{\pi}}\ar[d]_{\tau_1}&\widetilde{Y}\ar[d]^{\tau_2}\\
X\ar[r]_{\pi}&Y
}
\]
such that the following assertions hold.
\begin{enumerate}
\item[(1)] $\tau_1$ is a (crepant) terminalization and $\widetilde{X}$ has only $\mathbb{Q}$-factorial Gorenstein terminal singularities.
\item[(2)] $\widetilde{\pi}$ is an elementary  contraction of a $K_{\widetilde{X}}$-negative extremal ray, which is   divisorial.
\item[(3)] $Y$ has at worst $\mathbb{Q}$-factorial isolated canonical singularities.
\end{enumerate}
Suppose further that either $\pi$ maps the exceptional divisor $E:=\textup{Exc}(\pi)$ to a curve, or $\widetilde{\pi}$ maps the exceptional divisor $\widetilde{E}:=\textup{Exc}(\widetilde{\pi})$ to a single point.
Then we further have:
\begin{enumerate}
\item[(4)] $\widetilde{E}\cap\textup{Exc}(\tau_1)=\emptyset$ and $\widetilde{E}=\tau_1^{-1}(E)\cong E$;
\item[(5)]  $\tau_2$ is also crepant; and in particular, 
\item[(6)] if $\pi(E)$ is a curve, then $X$ is the blow-up of $Y$ along a local complete intersection curve $C$, $Y$ is  Gorenstein which is smooth around $C$, and $E$ is  Cartier; moreover, $\pi_*(-E|_E)=\pi(E)=C$.
\end{enumerate}
\end{lemme}

\begin{proof}
Let $\tau_1:\widetilde{X}\to X$ be a $\QQ$-factorial terminalization (cf. \cite[Corollary 1.4.3]{BCHM10}, by which $\tau_1$ is crepant), then $\widetilde{X}$ has only $\mathbb{Q}$-factorial Gorenstein terminal singularities.
Let $\widetilde{C}\subseteq\widetilde{X}$ be an irreducible curve such that $\tau_1(\widetilde{C})$ is $\pi$-contracted.
Then $K_{\widetilde{X}}\cdot \widetilde{C}=K_X\cdot\tau_1(\widetilde{C})<0$.
Therefore, there is an extremal ray $\widetilde{R}\in\overline{\textup{NE}}(\pi\circ\tau_1)\subseteq\overline{\textup{NE}}(\widetilde{X})$ such that $K_{\widetilde{X}}\cdot\widetilde{R}<0$.
Let $\widetilde{\pi}:\widetilde{X}\to \widetilde{Y}$ be the  contraction of $\widetilde{R}$.
By the rigidity lemma (cf.~\cite[Lemma 1.15, pp.~12-13]{Deb01}) $\pi\circ\tau_1$ factors through $\widetilde{\pi}$.
So $\widetilde{\pi}$ is birational and thus divisorial (see \cite[Theorem 4]{Kaw84} and \cite[Theorem 0]{Ben85}; cf.~\cite[Introduction]{Cut88}). 
Hence, (1) and (2) are proved. 
By {\hyperref[lem_del14]{Lemma  \ref*{lem_del14}}}, $\pi$ is  divisorial; hence (3) follows from \cite[Proposition 3.36]{KM98}, noting that non-terminal points of $Y$  are contained in the images of the non-terminal points of $X$ (cf. \cite[Corollary 3.43, pp.~104-105]{KM98}).
Let $\widetilde{F}$ be any curve contracted by $\widetilde{\pi}$ and set $F:=\tau_1(\widetilde{F})$.
Then $K_X\cdot F=K_{\widetilde{X}}\cdot\widetilde{F}<0$ implies that $F$ is still a curve and contracted by $\pi$.
%Hence, $(\tau_1)_*(\widetilde{R})$ is the extremal ray on $X$ contracted by $\pi$. 
Hence, $\tau_1(\widetilde{E})\subseteq E$, but $E$ being irreducible (since $\pi$ is elementary), this implies that $\tau_1(\widetilde{E})=E$.

From now on, we assume that either $\pi(E)$ is a curve or $\widetilde{\pi}(\widetilde{E})$ is a single point.
\textbf{We claim that $E$ does not contain any non-terminal point of $X$.}
Suppose the contrary.
Since $X$ is $\mathbb{Q}$-factorial, it follows from \cite[Corollary 2.63]{KM98} that $\textup{Exc}(\tau_1)$ is of pure codimension one.
Therefore, $\tau_1^*(E)=\widetilde{E}+F$ with $F$ being $\tau_1$-exceptional, noting that $\widetilde{E}$ is an irreducible divisor since $\widetilde\pi$ is elementary by (2).
Since $\widetilde{X}$ is also $\mathbb{Q}$-factorial, we take a curve $B$ in $\widetilde{E}\cap F$. Then from $K_{\widetilde{X}}\cdot B=\tau_1^*K_X\cdot B=0$ we see that $B$ is not contracted by $\widetilde\pi$, hence $\widetilde\pi(\widetilde B)$ is a curve and since $\widetilde E$ is irreducible we must have $\widetilde\pi(\widetilde E)=\widetilde\pi(B)$. 
If $\widetilde{E}$ is mapped onto a single point, then so is $B$, a contradiction.
If $E$ is mapped onto a curve, 
%Then with a similar argument, 
%$\widetilde{\pi}(\widetilde{E})=\widetilde{\pi}(B)$ is  a curve (i.e., $B$ is not $\widetilde{\pi}$-contracted); 
then $\widetilde{\pi}(\widetilde{E})=\widetilde{\pi}(B)$ is  contracted by $\tau_2$, implying that $\tau_2(\widetilde{\pi}(\widetilde{E}))$ is  a single point on $Y$, contradicting  the assumption that $\pi(E)$ is a curve.
So our claim holds and (4) is proved.
(5) follows from the the diagram (for some non-negative number $a$):
$$K_{\widetilde{Y}}=\widetilde{\pi}_*(K_{\widetilde{X}}-a\widetilde{E})=\widetilde{\pi}_*\tau_1^*\pi^*K_Y=\tau_2^*K_Y.$$
Now, we show (6). 
If $C:=\pi(E)$ is a curve, so is $\widetilde{\pi}(\widetilde{E})$; hence $K_{\widetilde{Y}}$ is Cartier
(cf.~\cite[Lemma 3]{Cut88}).
Since $\widetilde{E}$ is disjoint with $\textup{Exc}(\tau_1)$, we see that $\widetilde{X}$ and $X$ are isomorphic around $\widetilde{E}$, and hence $X$ is terminal around $E$.
Following from \cite[Corollary 3.43, pp.~104-105]{KM98}, $Y$ is also terminal around the image $C=\pi(E)$.
In addition, the restrictions $\widetilde{\pi}|_{\widetilde{E}}$ and $\pi|_E$ are the same contraction; therefore, $\widetilde{Y}$ and $Y$ are isomorphic around $\widetilde{C}$. 
By \cite[Theorem 4]{Cut88},  $X$ is the blow-up of a local complete intersection curve on $Y$ and $Y$ is smooth around $C$. 
Since $K_{\widetilde{Y}}=\tau_2^*K_Y$, our $K_Y$ is also Cartier: indeed, since $\tau_2$ is birational, the function field $K(\widetilde{Y})$  coincides with $K(Y)$; hence the local defining  equation for $K_{\widetilde{Y}}$ on $\widetilde{Y}$ is also that for $K_Y$. 
Applying {\hyperref[lem_del14]{Lemma  \ref*{lem_del14} (2)}} to $\pi$, we see that $E$ is also Cartier. 
Then  %$\mathcal{O}_X(-E)|_E=\mathcal{I}_E/\mathcal{I}_E^2|_E\cong\mathcal{O}_E(1)$, where $\mathcal{I}_E=\mathcal{O}_X(-E)$.
 $\mathcal{O}_X(-E)|_E\cong\mathcal{O}_E(1)$. 
Since $-E|_E$ is $\pi|_E$-ample, we have   $q(-E|_E)+G\sim H_E$ for some $q>0$, some fibre $G$ of $\pi|_E:E\to C$, and some very ample curve $H_E$ on $E$.
By the intersection theory and {\hyperref[lem_del14]{Lemma  \ref*{lem_del14}}}, $\deg (H_E\to C)=q$, so $(6)$ is proved.
\end{proof}

\begin{rmq}
If $\pi$ contracts $E$ to a point in {\hyperref[lem_canonical_terminal]{Lemma  \ref*{lem_canonical_terminal}}}, then  {\hyperref[lem_canonical_terminal]{Lemma  \ref*{lem_canonical_terminal} (4)}} may not be true, since $\widetilde{\pi}$ in this case will  possibly contract $\widetilde{E}$ to a curve, and then $\widetilde{E}$ is the blow-up of $E$ along some point; in other words, $E$ may contain some non-terminal point of $X$.
\end{rmq}

The following 
{\hyperref[contr_curve_elementary]{Proposition   \ref*{contr_curve_elementary}}} $\sim$ {\hyperref[prop_contr_surface_elementary]{Proposition   \ref*{prop_contr_surface_elementary}}} describe the first step of the MMP which is either a Fano contraction or a divisorial contraction mapping the exceptional divisor to a single point (cf.~{\hyperref[remark_conclude_excep_tocurve]{Remark  \ref*{remark_conclude_excep_tocurve}}}).

\begin{prop}\label{contr_curve_elementary}
Let $(X,\Delta)$ be a projective klt threefold pair, and $L_X$ a strictly nef divisor on $X$.
Suppose  $\rho(X)\leqslant 2$ (this is the case when $X$ admits a $(K_X+\Delta)$-negative  elementary contraction to a curve).
Then $K_X+\Delta+tL_X$ is ample for  $t\gg 1$.
\end{prop}
\begin{proof}
If view of  {\hyperref[mainthm-ample-3klt]{Theorem \ref*{mainthm-ample-3klt}}}, we may assume $\rho(X)=2$ and $K_X+\Delta$ is not parallel to $L_X$.  
Hence, the Mori cone $\overline{\textup{NE}}(X)$ has only two extremal rays. 
In particular, some linear combination $a(K_X+\Delta)+bL_X$ is strictly positive on $\overline{\textup{NE}}(X)\backslash \{0\}$ and thus ample (cf.~\cite[Theorem 1.18]{KM98}).
By {\hyperref[lem-big-ample]{Lemma  \ref*{lem-big-ample}}}, our proposition is proved.
\end{proof}

\begin{prop}\label{prop_Exc_surface_point}
Let $(X,\Delta)$ be a $\mathbb{Q}$-factorial normal  projective threefold with only  klt singularities and $L_X$ a strictly nef divisor.
Suppose there is a divisorial contraction $\pi:X\to X'$ of a $(K_X+\Delta)$-negative extremal ray, mapping the exceptional divisor to a point.	 
Then $K_X+\Delta+tL_X$ is ample for  $t\gg1$.
\end{prop}

\begin{proof}
In view of {\hyperref[lem-big-ample]{Lemma  \ref*{lem-big-ample}}}, we may assume that $K_X+\Delta+tL_X$ is not big.
By {\hyperref[lem-not-big-some]{Lemma  \ref*{lem-not-big-some}}}, $(K_X+\Delta)^i\cdot L_X^{3-i}=0$ for any $0\leqslant i\leqslant 3$.
Write $(K_X+\Delta)-aE=\pi^*(K_{X'}+\Delta')$ and $L_X+bE=\pi^*L_{X'}$ with $L_{X'}$ being  $\mathbb{Q}$-Cartier  (cf.~\cite[Theorem 3-2-1]{KMM87}) and $E$ being  $\pi$-exceptional. 
Since $-E$ is $\pi$-ample (cf.~\cite[Lemma 2.62]{KM98}) and $L_X$ is strictly nef, our $b>0$. 
By the projection formula, $L_{X'}$ is strictly nef.
Note that 
$\pi^*(K_{X'}+\Delta'+tL_{X'})=(K_X+\Delta+tL_X)+(bt-a)E$;  
hence for  $t\gg 1$, our $K_{X'}+\Delta'+tL_{X'}$ is strictly nef.

We claim that $K_{X'}+\Delta'+tL_{X'}$ is big (and hence ample by {\hyperref[lem-big-ample]{Lemma  \ref*{lem-big-ample}}}). 
Suppose the claim for the time being.
%Then there exists a suitable integer $m$, such that $|m(K_{X'}+\Delta'+tL_{X'})|$ is base point free (cf.~\cite[Theorem 3.3]{KM98}).
Fixing some $m\gg 1$, we choose a  smooth member $A\in |m(K_{X'}+\Delta'+tL_{X'})|$ which is ample.
Let $D_X:=b(K_X+\Delta)+aL_X$ and $D_{X'}:=b(K_{X'}+\Delta')+aL_{X'}$.
Then  $D_X=\pi^*(D_{X'})$.
Since $E$ is mapped to a point, $D_X^2\cdot(K_X+\Delta+tL_X)=0$ implies $D_{X'}^2\cdot(K_{X'}+\Delta'+tL_{X'})=0$.
Similarly, $D_{X'}\cdot (K_{X'}+\Delta'+tL_{X'})^2=D_X\cdot (K_X+\Delta+tL_X+(bt-a)E)^2=0$.  
So $D_{X'}^2\cdot A=D_{X'}\cdot  A^2=0$.
By \cite[Lemma 3.2]{Zha16}, we have $D_{X'}\equiv 0$. 
Then, $D_X\equiv0$ and   $-(K_X+\Delta)$ is parallel to $L_X$, which is strictly nef.
As a result, $-(K_X+\Delta)$ is ample (cf.~{\hyperref[mainthm-ample-3klt]{Theorem \ref*{mainthm-ample-3klt}}}) and our result follows.

It remains to show the bigness of $K_{X'}+\Delta'+tL_{X'}$.
Since $\pi(E)$ is  a single point, we have
%\begin{align*}
%	0\leqslant(K_{X'}+tL_{X'})^3&=\pi^*(K_{X'}+tL_{X'})^2\cdot ((K_X+tL_X)+(bt-a)E)\\
%	&=\pi^*(K_{X'}+tL_{X'})\cdot  ((K_X+tL_X)+(bt-a)E)\cdot (K_X+tL_X)\\
%	&=\pi^*(K_{X'}+tL_{X'})\cdot (K_X+tL_X)^2=(bt-a)(K_X+tL_X)^2\cdot E
%\end{align*}
$$0\leqslant(K_{X'}+\Delta'+tL_{X'})^3=\pi^*(K_{X'}+\Delta'+tL_{X'})\cdot (K_X+\Delta+tL_X)^2=(bt-a)(K_X+\Delta+tL_X)^2\cdot E.$$
Here, $-E$ is $\pi$-ample. 
Thus, $(L_X|_E)^2=L_X^2\cdot E=(\pi^*L_{X'}-bE)^2\cdot E=(-bE|_E)^2>0$.
By the  Nakai-Moishezon criterion (cf.~\cite[Theorem 1.37]{KM98}),  $L_X|_E$ is ample.
So the last item is positive for  $t\gg 1$.
In particular, $K_{X'}+tL_{X'}$ is big (cf.~\cite[Proposition 2.61]{KM98}).
\end{proof}

\begin{prop}%(cf.~\cite[Proposition 4.2]{CCP08}
\label{prop_contr_surface_elementary}
Let $X$ be a $\mathbb{Q}$-factorial normal projective threefold with only isolated  klt singularities,  and $L_X$ a strictly nef $\mathbb{Q}$-divisor on $X$.
Suppose  there is an elementary  $K_X$-negative contraction  $\pi:X\to S$ onto a normal projective surface $S$.
Then $K_X+tL_X$ is ample for $t\gg 1$.
\end{prop}

Before we enter the proof of {\hyperref[prop_contr_surface_elementary]{Proposition   \ref*{prop_contr_surface_elementary}}}, we extend a formula on conic bundles to  our singular case (cf.~{\hyperref[rem_composition_conic]{Remark  \ref*{rem_composition_conic}}} for a further extension  when $\rho(X/S)\geqslant 2$).

\begin{lemme}[{cf.~\cite[4.11]{Miy81}}]\label{lem_conic_miy}
Let $X$ be a normal projective threefold with at worst isolated klt singularities.
Suppose that $\pi:X\to S$ is an elementary  $K_X$-negative contraction  onto a normal projective surface $S$.
Denote by $D_1$ the one-dimensional part of the discriminant locus of $\pi$ (over which, $\pi$ is not smooth).
Then $\pi_*K_X^2\equiv -(4K_S+D_1)$.
\end{lemme}

\begin{proof}
Since $\rho(X/S)=1$, by the  canonical bundle formula (cf.\,e.g.~\cite[Theorem 0.2]{Amb05}), there exists some  $\Delta_S\geqslant 0$ on $S$ such that $(S,\Delta_S)$ is klt and thus $S$ is $\mathbb{Q}$-factorial (cf.~e.g.~\cite[Proposition 4.11]{KM98}), and
%has only rational singularities (cf.~\cite[Theorem 5.22]{KM98}).
%Then, $S$ is $\mathbb{Q}$-factorial (cf.~\cite[Proposition 17.1]{Lip69}), and 
we only need to check the equality  on very ample curves  on $S$. % by Bertini's theorem.
%Now we note that if E is very ample on X then almost all curves E' in the complete linear system |E| are smooth by embedding X into some Pn using E and then applying Bertini's Theorem (Hartshorne, Thm. II.8.18). 
%We include the proof here for readers' convenience. 
%First, our $S$ is $\mathbb{Q}$-factorial (cf.~\cite[Proposition 17.1]{Lip69}).
By the cone theorem (cf.~\cite[Theorem 3.7]{KM98}), $\pi$ is equi-dimensional.
By \cite[Theorem 5.10]{KM98}, $X$ is Cohen-Macaulay.
Let $D_0:=(\textup{Sing}~S)\cup\pi(\textup{Sing}~X)$.
Then, $\pi|_{X\backslash\pi^{-1}(D_0)}$ is flat %(cf.~\cite[Theorem 23.1 and its Corollary]{Mat89}) 
and thus $\pi|_{X\backslash\pi^{-1}(D_0)}$ is a usual conic bundle  (cf.~\cite[(1.5)]{Sar82}).  
Let $T$ be a very ample curve on $S$ which can be assumed to be smooth, avoid $D_0$, and intersect with $D_1$ transversally. 
Let $F:=\pi^{-1}(T)=\pi^*(T)$, which is smooth.
Then 
$$K_X^2\cdot F=(K_X|_F)^2=(K_F-F|_F)^2=K_F^2-2K_F\cdot (F|_F)=K_F^2+4T^2.$$ 
Note that the last equality is due to the adjunction.
Since $F$ is a (not necessarily minimal) ruled surface over $T$ with $D_1
\cdot T$ degenerate  (reducible) fibres, we have
$$K_F^2=-4(K_S\cdot T+T^2)-D_1\cdot T.$$ 
As a result, we have $\pi_*(K_X^2)\cdot T=K_X^2\cdot F=-(4K_S+D_1)\cdot T$.
So our lemma is proved.
\end{proof}

\begin{proof}[Proof of {\hyperref[prop_contr_surface_elementary]{Proposition   \ref*{prop_contr_surface_elementary}}}]
Let us assume that $L_X$ is Cartier after replacing $L_X$ by a multiple. 
By {\hyperref[coro_q0>0]{Corollary   \ref*{coro_q0>0}}}, {\hyperref[lem_strict_nef_k]{Lemma  \ref*{lem_strict_nef_k}}} and {\hyperref[lem-big-ample]{Lemma  \ref*{lem-big-ample}}}, we may assume $q^\circ(X)=0$, and $K_X+tL_X$ is nef but not big for  $t\gg 1$. 
%Then  $K_X^3=K_X^2\cdot L_X=K_X\cdot L_X^2=L_X^3=0$ (cf.~).
Note that we can further assume $K_X$ not parallel to $L_X$ (cf.~{\hyperref[mainthm-ample-3klt]{Theorem \ref*{mainthm-ample-3klt}}}).  
By the canonical bundle formula (cf.~e.g. \cite[Theorem 0.2]{Amb05}), $(S,\Delta_S)$ is a klt pair for some effective divisor $\Delta_S$ on $S$; thus $S$ is $\mathbb{Q}$-factorial (cf.~e.g.~\cite[Proposition 4.11]{KM98}).
Let $u:=\frac{-K_X\cdot f}{L_X\cdot f}>0$ (which is a rational number) where $f$ is a general fibre of $\pi$.
By the cone theorem (cf.~\cite[Theorem 3.7]{KM98}), there exists a $\mathbb{Q}$-Cartier divisor $M$ such that
$K_X+uL_X=\pi^*M$ with $M\not\equiv 0$.  
Then, {\hyperref[lem-not-big-some]{Lemma  \ref*{lem-not-big-some}}} gives us 
\begin{align*}
0=(K_X-\pi^*M)^3=-3K_X^2\cdot(K_X+uL_X)+3K_X\cdot(\pi^*M)^2=3(K_X\cdot f)M^2,
\end{align*}
which implies  $M^2=0$.  
Fix a rational number $t>6$ such that  $K_X+tL_X$ is strictly nef.  
By {\hyperref[lem-not-big-some]{Lemma  \ref*{lem-not-big-some}}},  there exists  $\alpha\in\overline{\textup{ME}}(X)$ such that $K_X\cdot\alpha=L_X\cdot \alpha=0$.
Then $M\cdot \gamma=0$ with $0\not\equiv\gamma:=\pi_*\alpha\in\overline{\textup{ME}}(S)$.
Since $\dim S=2$, our $\gamma$ is nef.
%Replacing $\gamma$ by a multiple $G$, we may assume that $G$ is an integral nef Cartier divisor satisfying $M\cdot G=0$. 
Since $M^2=0$ but $M\not\equiv0$, we have $\gamma^2=0$ and thus $\gamma$ is parallel to $M$ by the Hodge index theorem. 
%Let $H$ be an ample divisor on $S$. 
%Since $\gamma^2=M^2=0$ but neither of them are trivial, our $H\cdot \gamma\neq 0$ and $H\cdot M\neq 0$.
%Take $P:=(H\cdot \gamma)M-(H\cdot M)\gamma$. 
%Then $P^2=H\cdot P=0$.
%By the Hodge index theorem again, $P\equiv 0$ and $\gamma$ is parallel to $M$, which implies that 
Hence, either $M$  is nef or $-M$ is nef.
Denote by $M_1=M$ (resp. $-M$) if $M$ is nef (resp. $-M$ is nef). 
Replacing $M_1$ by a multiple, we may assume that $M_1$ is a line bundle.

\begin{claim}\label{claim_m-k-pseu}
$N:=M-K_S$	is pseudo-effective.
\end{claim}

\noindent
\textbf{Proof of  {\hyperref[claim_m-k-pseu]{Claim \ref*{claim_m-k-pseu}}}.}
For any irreducible curve $\ell\subseteq S$, it follows from {\hyperref[lem_conic_miy]{Lemma    \ref*{lem_conic_miy}}} that
\begin{align*}
 0\leqslant  u^2L_X^2\cdot\pi^*(\ell)&=(\pi^*M-K_X)^2\cdot\pi^*(\ell)=-2\pi^*M\cdot K_X\cdot \pi^*(\ell)	+K_X^2\cdot\pi^*(\ell)\\
 &=-2(K_X\cdot f)M\cdot \ell-(4K_S+D_1)\cdot \ell=(4N-D_1)\cdot \ell.
\end{align*}
Here,  $D_1$ denotes the one-dimensional part of the discriminant locus of  $\pi$.  
%Then any nef divisor $G\in\textup{Nef}(S)=\overline{\textup{ME}}(S)$, which is a limit of movable curves, also satisfies $(4N-D_1)\cdot G\geqslant 0$.
Then $4N-D_1$ is nef and hence
$N=\frac{1}{4}((4N-D_1)+D_1)$ is pseudo-effective.

\par \vskip 1pc \noindent

We come back to the proof of {\hyperref[prop_contr_surface_elementary]{Proposition   \ref*{prop_contr_surface_elementary}}}. 
Let $\tau:\widetilde{S}\to S$ be a minimal resolution, and  $\widetilde{M_1}:=\tau^*M_1$. % and $\widetilde{N}=\pi^*N$.
Since  $M_1\cdot M=0$ and $M_1\cdot N\geqslant 0$ (cf.~{\hyperref[claim_m-k-pseu]{Claim \ref*{claim_m-k-pseu}}}), our $K_{\widetilde{S}}\cdot \widetilde{M_1}=K_S\cdot M_1\leqslant 0$. 
Then, for any positive integer $n$, applying the Riemann-Roch formula to $n\widetilde{M_1}$ and noting that $q(\widetilde{S})=q(S)=q(X)=0$, we get the following inequality
\begin{align}\label{eq_RR}
\begin{split}
h^0(S,nM_1)&=h^0(\widetilde{S},n\widetilde{M_1})=-\frac{n}{2}\widetilde{M_1}\cdot K_{\widetilde{S}}+\chi(\mathcal{O}_{\widetilde{S}})+h^1(\widetilde{S},n\widetilde{M_1})-h^2(\widetilde{S},n\widetilde{M_1})\\
&\geqslant 1-h^2(\widetilde{S},n\widetilde{M_1}).
\end{split}
\end{align}

\textbf{We claim that $h^2(\widetilde{S},n\widetilde{M_1})=h^0(K_{\widetilde{S}}-n\widetilde{M_1})=0$ for $n\gg 1$.}  
Fixing an ample divisor $\widetilde{H}$ on $\widetilde{S}$, we have $\widetilde{M_1}\cdot \widetilde{H}>0$ by the Hodge index theorem (noting that $\widetilde{M_1}^2=M_1^2=0$).
For each $n$, if there is an effective divisor $Q_n$  on $\widetilde{S}$ such that $K_{\widetilde{S}}-n\widetilde{M_1}\sim Q_n$, then 
$$K_{\widetilde{S}}\cdot \widetilde{H}=(n\widetilde{M_1}+Q_n)\cdot\widetilde{H}\geqslant  n\widetilde{M_1}\cdot\widetilde{H}.$$
The left hand side of the above inequality being bounded, our claim is thus proved.

Therefore, it follows from {\hyperref[eq_RR]{Equation  (\ref*{eq_RR})}}  that $M_1$ is numerically equivalent to an effective $\mathbb{Q}$-divisor, which is non-zero by our assumption in the beginning of the proof.
This implies that 
 $K_X+uL_X$ (or $-K_X-uL_X$) is  numerically equivalent to  a non-zero effective divisor. 
By {\hyperref[prop-q-effective]{Proposition  \ref*{prop-q-effective}}}, our proposition is proved.
\end{proof}

The following theorem generalizes {\hyperref[prop_contr_surface_elementary]{Proposition   \ref*{prop_contr_surface_elementary}}} to the non-elementary case.

\begin{thm}\label{thm_contr_surface_conic}
Let $X$ be a $\mathbb{Q}$-factorial Gorenstein normal projective threefold with only isolated  canonical singularities,  and $L_X$ a strictly nef divisor on $X$.
Suppose that $X$ admits an equi-dimensional  $K_X$-negative contraction (of an extremal face) $\pi:X\to S$ onto a normal projective surface such that $K_X+uL_X=\pi^*M$ for some $u\in\mathbb{Q}$ and some $\mathbb{Q}$-Cartier divisor $M$ on $S$.
%Suppose further that $\pi$ is equi-dimensional.
Then $K_X+tL_X$ is ample for $t\gg 1$.
\end{thm}

\begin{rmq}\label{rem_composition_conic}
With the same assumption as in {\hyperref[thm_contr_surface_conic]{Theorem    \ref*{thm_contr_surface_conic}}},  applying \cite[Proof of Proposition 3.4]{Rom19} and {\hyperref[lem_del14]{Lemma  \ref*{lem_del14}}}, we 
get the following MMP for $X$ over $S$, noting that the Gorenstein condition on $X$ can descend to each $X_i$ (cf.~{\hyperref[lem_canonical_terminal]{Lemma  \ref*{lem_canonical_terminal} (6)}}).
\[\xymatrix{X=:X_0\ar[r]^{\phi_0}\ar[drrr]_{\pi_0:=\pi}&X_1\ar[r]^{\phi_1}&\cdots\ar[r]^{\phi_{n-1}}&X_n\ar[d]^{\pi_n}\\
&&&S
}
\]
Here, each $\phi_i$ is an elementary $K_{X_i}$-negative divisorial contraction mapping the exceptional divisor  onto a curve (cf.~{\hyperref[lem_del14]{Lemma  \ref*{lem_del14}}}), each $X_i$ is a normal projective threefold with only isolated $\mathbb{Q}$-factorial Gorenstein canonical singularities  (cf.~{\hyperref[lem_canonical_terminal]{Lemma  \ref*{lem_canonical_terminal}}}), and $\pi_n$ is an elementary conic fibration in the sense that the generic fibre is a smooth plane conic. 

With this kept in mind, we can extend the formula in {\hyperref[lem_conic_miy]{Lemma   \ref*{lem_conic_miy}}} to the non-elementary case in our situation.
Let $\phi:=\phi_{n-1}\circ\cdots\circ\phi_0$.
By {\hyperref[lem_del14]{Lemma  \ref*{lem_del14} (2)}} and {\hyperref[lem_canonical_terminal]{Lemma  \ref*{lem_canonical_terminal} (6)}},  $K_X=\phi^*K_{X_n}+\sum E_i$ with $E_i$  being pairwise disjoint, and $\phi_*(-E_i|_{E_i})=\phi(E_i)$.
Then for any divisor $H$ on $X_n$, we have 
\begin{align*}
	\phi_*(K_X^2)\cdot H&=(\phi^*K_{X_n}\cdot\phi^*K_{X_n}+2\sum\phi^*K_{X_n}\cdot E_i+\sum E_i|_{E_i})\cdot \phi^*H\\
	&=K_{X_n}^2\cdot H-\sum \phi(E_i)\cdot H
\end{align*}
where $\phi(E_i)$ are pairwise disjoint  curves, and all of them are not $\pi_n$-contracted. 
Combining the above numerical equivalence with {\hyperref[lem_conic_miy]{Lemma    \ref*{lem_conic_miy}}}, we have 
$\pi_*(K_X^2)\equiv (\pi_n)_*(K_{X_n}^2)-\sum a_i\pi(E_i)=:-(4K_S+D)$,
where each $a_i>0$, and $D$ is the sum of the one-dimensional part of the discriminant locus of $\pi_n$ and $\sum a_i\pi(E_i)$; hence, $D$ is  effective.
\end{rmq}

\begin{proof}[Proof of {\hyperref[thm_contr_surface_conic]{Theorem    \ref*{thm_contr_surface_conic}}}]
The  proof is completely the same as {\hyperref[prop_contr_surface_elementary]{Proposition   \ref*{prop_contr_surface_elementary}}} after replacing {\hyperref[lem_conic_miy]{Lemma    \ref*{lem_conic_miy}}} by {\hyperref[rem_composition_conic]{Remark  \ref*{rem_composition_conic}}}.
\end{proof}

%We end up this section with the following remark.
\begin{rmq}\label{remark_conclude_excep_tocurve}
We shall finish the proof of  {\hyperref[main_theorem_Goren_ter_3fold]{Theorem   \ref*{main_theorem_Goren_ter_3fold} (3)}}.  %(cf.~{\hyperref[thm_3fold_surface_curve]{Theorem \ref*{thm_3fold_surface_curve}}}).
%By , such $X$ does not admit any small contractions.
In view of {\hyperref[lem_del14]{Lemma  \ref*{lem_del14}}} and {\hyperref[contr_curve_elementary]{Proposition   \ref*{contr_curve_elementary}}}  $\sim$ {\hyperref[prop_contr_surface_elementary]{Proposition   \ref*{prop_contr_surface_elementary}}}  above,  we only need to verify the case when all the elementary $K_X$-negative  contractions (of extremal rays) are divisorial contractions, mapping the exceptional divisors to curves, % (cf.~\cite[Proposition 5.2]{CCP08}). 
which is {\hyperref[thm_3fold_surface_curve]{Theorem \ref*{thm_3fold_surface_curve}}}.
\end{rmq}

\begin{thm}[{cf.~\cite[Proposition 5.2]{CCP08}}]\label{thm_3fold_surface_curve}
Let  $X$ be a  $\mathbb{Q}$-factorial Gorenstein normal projective uniruled threefold with only isolated  canonical singularities, 
and $L_X$ a strictly nef divisor.
Suppose  all the elementary $K_X$-negative extremal contractions  are divisorial, mapping the exceptional divisors to curves.
Then $K_X+tL_X$ is ample for $t\gg 1$.
\end{thm}

From now on till the end of the appendix, let us show {\hyperref[thm_3fold_surface_curve]{Theorem \ref*{thm_3fold_surface_curve}}}.

\begin{notation}\label{not_bir_surface_curve}
We shall always stick to the following notations 
 and apply the induction on the Picard number $\rho(X)$. 
\begin{enumerate}
\item[(1)] In view of {\hyperref[main_theorem_Goren_ter_3fold]{Theorem   \ref*{main_theorem_Goren_ter_3fold} (2)}}, we may assume the augmented irregularity $q^\circ(X)=0$.
\item[(2)] Let $\varphi_i:X\to X_i$ be the contraction of the $K_X$-negative extremal ray $\mathbb{R}_{\geqslant 0}[\ell_i]$, with the exceptional divisor $E_i$ mapped to a (possibly singular) curve $C_i$ on $X_i$. 
Let $\ell_i\cong\mathbb{P}^1$ be the general fibre such that $K_X\cdot\ell_i=E_i\cdot \ell_i=-1$ (cf.~{\hyperref[lem_del14]{Lemma  \ref*{lem_del14}}}).
\item[(3)] By {\hyperref[lem_canonical_terminal]{Lemma  \ref*{lem_canonical_terminal}}}, each $X_i$ also has at worst isolated $\mathbb{Q}$-factorial Gorenstein canonical singularities  with $\rho(X_i)=\rho(X)-1$.
\item[(4)] Let $I$ be the index recording the elementary $K_X$-negative extremal contractions.
\item[(5)] Let $\nu:=\min\left\{\frac{L_X\cdot\ell_i}{-K_X\cdot\ell_i}~|~i\in I\subseteq\mathbb{N}\right\}=\min\{L_X\cdot\ell_i~|~i\in I\}$.
Then $D_X:=L_X+\nu K_X$ is nef.
In view of {\hyperref[mainthm-ample-3klt]{Theorem \ref*{mainthm-ample-3klt}}}, we may assume that $D_X\not\equiv 0$.
\item[(6)] Let $I_0\subseteq I$ be the subset such that $i\in I_0$ if and only if $L_X\cdot \ell_i=\nu$.
\item[(7)] Let $\varphi=\varphi_1:X\to X_1=:X'$, $E:=E_1$, $L_{X'}:=\varphi_*L_X$ and $C':=\varphi(E)$ with $1\in I_0$. 
\item[(8)] Write $K_X=\varphi^*K_{X'}+E$, and $L_X=\varphi^*L_{X'}-\nu E$ (cf.~{\hyperref[lem_del14]{Lemma  \ref*{lem_del14}}}).
Let $D_{X'}:=L_{X'}+\nu K_{X'}$.
Then $D_X=\varphi^*D_{X'}$ and thus $D_{X'}$ is also nef.
\end{enumerate}	
\end{notation}
%Note that when $\rho(X)=1$, our $K_X+tL_X$ is clearly ample for $t\gg 1$.

\textbf{Now we begin to prove {\hyperref[thm_3fold_surface_curve]{Theorem \ref*{thm_3fold_surface_curve}}}. 
If $\rho(X)\leqslant 2$, then our theorem follows from {\hyperref[contr_curve_elementary]{Proposition   \ref*{contr_curve_elementary}}}.
Suppose that our theorem holds for the case $\rho(X)\leqslant p$.
We shall assume $\rho(X)=p+1$ in the following.}
%\begin{hyp}\label{assumption_absurd}
%Theorem \ref{thm_3fold_surface_curve} does not hold when $\rho(X)=p$, i.e., $K_X+tL_X$ is not ample for all $t\gg 1$. 
%Then it follows from Proposition \ref{prop-q-effective} that $D_X$ is not equivalent to an effective divisor (and hence not big).
%\end{hyp}

\begin{lemme}\label{lem_L.C>0}
Either $K_X+tL_X$ is ample for $t\gg 1$, or $L_{X'}\cdot C'\leqslant 0$.
\end{lemme}
\begin{proof}
Suppose the contrary that $K_X+tL_X$ is not ample for any $t\gg 1$ and $L_{X'}\cdot C'>0$. 
Then $L_{X'}$ is strictly nef on $X'$ and $K_{X'}+tL_{X'}$ is ample for  $t\gg 1$ by the induction on $\rho(X')$ (cf.~{\hyperref[remark_conclude_excep_tocurve]{Remark  \ref*{remark_conclude_excep_tocurve}}}). 
\textbf{We claim that $D_{X'}$ is semi-ample.} 
Consider the following 
$$\frac{2}{\nu}D_{X'}-K_{X'}=2(K_{X'}+\frac{1}{\nu}L_{X'})-K_{X'}=(K_{X'}+\frac{3}{2\nu}L_{X'})+\frac{1}{2\nu}L_{X'}.$$
Since $K_{X'}+\frac{3}{2\nu}L_{X'}=\frac{1}{\nu}D_{X'}+\frac{1}{2\nu}L_{X'}$ with $D_{X'}$ and $L_{X'}$ being nef, it must be big, for otherwise, $D_{X'}^3=D_{X'}^2\cdot L_{X'}=D_{X'}\cdot L_{X'}^2=L_{X'}^3=0$ would imply  $(K_{X'}+tL_{X'})^3=0$, a contradiction.
Hence, $\frac{2}{\nu}D_{X'}-K_{X'}$ is nef and big.
By the base-point-free theorem (cf.~\cite[Theorem 3.3]{KM98}), 
$D_{X'}$ is semi-ample. 
By {\hyperref[not_bir_surface_curve]{Notation  \ref*{not_bir_surface_curve} (5)}}
 and {\hyperref[prop-q-effective]{Proposition  \ref*{prop-q-effective}}}, our $K_X+tL_X$ is ample for $t\gg 1$,  a contradiction.
\end{proof}

\begin{lemme}\label{lem_D.C>0}
Either $K_X+tL_X$ is ample for $t\gg 1$, or $D_{X'}\cdot C'>0$.	
\end{lemme}

\begin{proof}
Suppose the contrary that $K_X+tL_X$ is not ample for any $t\gg 1$, and $D_{X'}\cdot C'=0$. 
Then $K_{X'}\cdot C'\geqslant 0$ (cf.~{\hyperref[lem_L.C>0]{Lemma \ref*{lem_L.C>0}}}); hence $(K_X-E)|_E=\varphi^*K_{X'}|_E$ is a nef divisor on $E$ (cf.~{\hyperref[lem_del14]{Lemma  \ref*{lem_del14}}} and {\hyperref[not_bir_surface_curve]{Notation  \ref*{not_bir_surface_curve} (5)}}).
Besides, $D_{X'}\cdot C'=0$ implies that our $D_X|_E\equiv 0$;  hence $L_X|_E\equiv-\nu K_X|_E$. 
So our $-K_X|_E$ is strictly nef on $E$.  
Together with the nefness of $(K_X-E)|_E$,
our $-E|_E$ is also strictly nef on $E$. %, noting that $K_X=\varphi^*K_{X'}+E$ and for any horizontal curve $B\subseteq E$ of $\varphi$, we have  $\varphi_*B=aC$ for some $a>0$.
%Since $L_{X'}\cdot B>0$ for every irreducible curve $B\neq C$, our $C$ cannot move. 
%$\varphi$ is the blow-up of a reduced and irreducible curve $C$ on $X'$.
%Hence, 
%We note that every horizontal curve of $X$ dominating $C$ is not contained in  $\textup{Sing}\,(E)$ (cf.~Lemma \ref{lem_del14}).
We consider the following  diagram.
\[\xymatrix@C=5em{
\widetilde{E}\ar[r]^\sigma\ar[d]_\tau\ar[dr]^q&E_N\ar[r]^{p_N}\ar[d]^{n_E}&C'_N\ar[d]^{n_{C'}}\\
\widetilde{E}_m\ar[d]&E\ar[r]^p\ar@{^(->}[d]&C'\ar@{^(->}[d]\\
C'_N&X\ar[r]^\varphi&X'
}
\]
Here, $p:=\varphi|_E$, $n_\bullet$ is the normalization, $\sigma$ is the minimal resolution, $\tau$ is the MMP of $\widetilde{E}$, $p_N$ is the induced map and $q:=n_E\circ\sigma$.
Then, $\widetilde{E}_m$ is a ruled surface. 
Denote by $C_0\subseteq \widetilde{E}_m$ the section with the minimal self-intersection $(C_0)^2=-e$, and
$f$ a general fibre of $\widetilde{E}_m\to C_N'$.
%Since both $X$ and $X'$ are Gorenstein, we have
%$$K_X=\varphi^*K_{X'}+E,~L_X=\varphi^*L_{X'}-\nu E.$$

As is shown in  {\hyperref[prop_Q-Goren_surface]{Proposition  \ref*{prop_Q-Goren_surface}}}, $K_{\widetilde{E}}\sim_{\mathbb{Q}}q^*K_E-F$, where $F$ is an effective divisor with $\varphi(q(F))\subseteq \textup{Sing}\,(C')$ (cf.~\cite[Lemma 5-1-9]{KMM87}, \cite[(4.1)]{Sak84} and {\hyperref[lem_del14]{Lemma  \ref*{lem_del14}}}).
Let $\widetilde{C}\subseteq \widetilde{E}$ be the strict transform of $C_0$  and $C_X:=q(\widetilde{C})$.
Since $C_X\not\subseteq\textup{Sing}\,E$ (cf.~{\hyperref[lem_del14]{Lemma  \ref*{lem_del14}}}),
%one can regard $\widetilde{C}\subseteq\widetilde{E}$ as the proper transform of $C_X$ along $q$ since the morphism $q$ is an isomorphism in the generic point of $C_X$.
$q$ is isomorphic in the generic point of $C_X$ and  $\widetilde{C}\not\subseteq\textup{Supp}\,F$. 
%By the projection formula,
Then we have
\begin{equation}\label{equ_deform}
K_{\widetilde{E}}\cdot \widetilde{C}\leqslant K_E\cdot C_X=(K_X+E)\cdot C_X\leqslant -2,	
\end{equation}
since both $K_X$ and $E$ are Cartier (cf.~{\hyperref[lem_canonical_terminal]{Lemma  \ref*{lem_canonical_terminal}}}). 
By \cite[Chapter 2, Theorem 1.15]{Kollar96},  
%we have 
$$\dim_{\widetilde{C}}\textup{Chow}(\widetilde{E})\geqslant -K_{\widetilde{E}}\cdot \widetilde{C}-\chi(\mathcal{O}_{\widetilde{C}_N})\geqslant -K_{\widetilde{E}}\cdot \widetilde{C}-1\geqslant 1,$$
where  $\widetilde{C}_N$ is the normalization of $\widetilde{C}$.
Then, $\widetilde{C}$ (and hence its push-forward $\tau_*(\widetilde{C})=C_0$) deforms, which  implies $e\leqslant 0$.
Let us consider the following equalities, noting that $-K_X\cdot \ell=-E\cdot \ell=1$ for a general fibre $\ell\subseteq E$ of $\varphi$.
\begin{align*}
	&q^*(-K_X|_E)=\tau^*(C_0+\alpha f)+\sum a_iP_i,\\
	&q^*(-E|_E)=\tau^*(C_0+\beta f)+\sum b_iP_i,\\
	&q^*(-K_E)=\tau^*(2C_0+(\alpha+\beta)f)+\sum(a_i+b_i)P_i,\\
	&q^*((K_X-E)|_E)=\tau^*((\beta-\alpha)f)+\sum(b_i-a_i)P_i,
\end{align*}
with $P_i$ being $\tau$-exceptional.
%Note that the coefficient of $C_0$ in each equality is deduced  from the projection formula by intersecting  with $\tau^*(f)$. 
On the one hand, the strict nefness of $-K_X|_E$ and $-E|_E$ gives  that $q^*(-K_X|_E)\cdot \tau^*(C_0)>0$ and $q^*(-E|_E)\cdot \tau^*(C_0)>0$; hence $\alpha-e>0$ and $\beta-e>0$.
On the other hand, since $\varphi^*K_{X'}|_E=(K_X-E)|_E$ is nef, we have $\beta-\alpha=q^*((K_X-E)|_E)\cdot \tau^*(C_0)\geqslant  \varphi^*K_{X'}|_E\cdot C_X\geqslant 0$ \hypertarget{1ag}{\textbf{(\dag)}}.

Since $K_{\widetilde{E}}\sim_{\mathbb{Q}}q^*K_E-F$,
there is an inclusion of the canonical sheaf $\omega_{\widetilde{E}}\subseteq q^*(\omega_E)$ as shown in {\hyperref[prop_Q-Goren_surface]{Proposition  \ref*{prop_Q-Goren_surface}}} (cf.~ \cite[Lemma 5-1-9]{KMM87} and \cite[(4.1)]{Sak84}); hence  we have 
$\omega_{\widetilde{E}_m}=\tau_*(\omega_{\widetilde{E}})\subseteq (\tau_*q^*(\omega_E))^{\vee\vee}$. 
Consequently, we get the following inequality 
$$-2C_0-(\alpha+\beta)f\geqslant -2C_0+(2g-2-e)f,$$ 
with $g=g(C_0)$ being the genus.  
So $\alpha+\beta+2g-2-e\leqslant 0$ \hypertarget{2ag}{\textbf{(\dag\dag)}}.
Furthermore,  $C_0+\alpha f$  being  strictly nef on $\widetilde{E}_m$ by the projection formula, 
 we  have $(C_0+\alpha f)^2\geqslant 0$. 
This gives that $\alpha\geqslant e/2$.
Together with \hyperlink{1ag}{\textbf{(\dag)}} and \hyperlink{2ag}{\textbf{(\dag\dag)}}, our $g\leqslant 1$.

It is known that strictly nef divisors on (minimal) ruled surfaces over curves of genus $\leqslant 1$ are indeed ample (cf.\,e.g.\,\cite[Example 1.23 (1)]{KM98}).
Therefore, $(C_0+\alpha f)^2>0$, and thus $\beta\geqslant  \alpha>e/2$ (cf.~\hyperlink{1ag}{\textbf{(\dag)}}).
Return back to \hyperlink{2ag}{\textbf{(\dag\dag)}}, we have $g<1$.
So $g=0$ and $C_0\cong\mathbb{P}^1$.
Since $C_0$ deforms, we have $e=0$, $\widetilde{E}_m\cong\mathbb{P}^1\times\mathbb{P}^1$ and $\alpha+\beta\leqslant 2$ (cf.~\hyperlink{2ag}{\textbf{(\dag\dag)}}). 
Since  $K_X$ is Cartier, both $\alpha$ and $\beta$ are positive integers; hence $\alpha=\beta=1$.
Then we have \hypertarget{1*}{\textbf{(*)}}: $\varphi^*K_{X'}|_E=(K_X-E)|_E\equiv 0$ (cf.~\hyperlink{1ag}{\textbf{(\dag)}}), and thus $\varphi^*L_{X'}|_E\equiv 0$.
%Then $K_{X'}\cdot C=L_{X'}\cdot C=0$ by \textbf{(\dag)} and our assumption $D_{X'}\cdot C=0$ in the beginning. 
%Also, we have $K_X\cdot C_X=E\cdot C_X=-1$. 
%Together with $K_{\widetilde{E}}\sim_{\mathbb{Q}}q^*K_E-F$, we have  $K_{\widetilde{E}}\cdot\widetilde{C}\leqslant K_E\cdot C_X=-2$.
%So applying the adjunction formula, we get $\widetilde{C}^2\geqslant 0$.

\textbf{We claim  that $\tau$ is an isomorphism.} 
Suppose  $\tau^*(C_0)=\widetilde{C}+\sum P_i$ with $P_i$ being $\tau$-exceptional.
Here, our $C_0$ can be chosen as any horizontal section containing some blown-up points of $\tau$ since $\widetilde{E}_m\cong\mathbb{P}^1\times\mathbb{P}^1$.
Then it follows from the projection formula that $\widetilde{C}^2<C_0^2=0$, a contradiction to  {\hyperref[equ_deform]{Equation  (\ref*{equ_deform})}}. 
So $\tau$ is isomorphic as claimed.

Now that $L_{X'}$ is nef, for $t\gg 1$, $K_{X'}+tL_{X'}$ is nef by the projection formula, noting that $\varphi^*(K_{X'}+tL_{X'})=(K_X+tL_X)+(\nu t-1)E$ and $\varphi^*K_{X'}|_E\equiv \varphi^*L_{X'}|_E\equiv 0$ as shown in \hyperlink{1*}{\textbf{(*)}}.
If $K_{X'}+tL_{X'}$ is  big for $t\gg 1$, then 
with the same proof of {\hyperref[lem_L.C>0]{Lemma \ref*{lem_L.C>0}}}, our $K_X+tL_X$ is ample, contradicting our assumption.
So we have $(K_{X'}+tL_{X'})^3=0$ for any $t\gg 1$. 
This in turn implies $K_{X'}^3=0$. 
On the other hand, we note that $K_X^3=0$ (cf.~{\hyperref[lem-big-ample]{Lemma  \ref*{lem-big-ample}}}). 
So we  get a contradiction (cf.~\hyperlink{1*}{\textbf{(*)}} and {\hyperref[lem_canonical_terminal]{Lemma  \ref*{lem_canonical_terminal} (6)}}):
$$0=K_X^3=(\varphi^*K_{X'}+E)^3=E^3=(q^*(E|_E))^2=(C_0+f)^2=2.$$
So our lemma is proved.
\end{proof}

\begin{lemme}\label{lem_intersect_C_<-1}
Suppose that $K_X+tL_X$ is not ample for any $t\gg 1$.
Then, for any curve $B'\subseteq X'$ such that $D_{X'}\cdot B'=0$, we have $K_{X'}\cdot B'\leqslant -1$.
In particular, if $B'\cap C'\neq\emptyset$ (as sets), then $K_{X'}\cdot B'\leqslant -2$.
\end{lemme}

\begin{proof}
By {\hyperref[lem_D.C>0]{Lemma \ref*{lem_D.C>0}}}, $B'\neq C'$.
Denote by $\hat{B'}$ the $\varphi$-proper transform of $B'$ on $X$.	
Then $D_X\cdot \hat{B'}=0$ and thus $K_{X}\cdot \hat{B'}\leqslant -1$, noting that $L_X$ is strctly nef and  $K_X$ is Cartier (cf.~{\hyperref[lem_canonical_terminal]{Lemma  \ref*{lem_canonical_terminal}}}).
Since $E\cdot \hat{B'}\geqslant 0$, we see that $K_{X'}\cdot B'=(K_X-E)\cdot \hat{B'}\leqslant -1$.
In particular, if $B'\cap C'\neq\emptyset$, then $E\cdot \hat{B'}\geqslant 1$, and hence $K_{X'}\cdot \hat{B'}\leqslant -2$. 
\end{proof}

\begin{lemme}\label{lem_not_big_X'}
Either $K_X+tL_X$ is ample for $t\gg 1$, or $D_{X'}$ is not strictly nef.
In the latter case, there is an extremal ray $\mathbb{R}_{\geqslant 0}[\ell']$ on $X'$ such that $K_{X'}\cdot\ell'<0$ and $D_{X'}\cdot \ell'=0$.
\end{lemme}

\begin{proof}
We may assume that $K_X+tL_X$ is not ample for any $t\gg 1$. 
Suppose that $D_{X'}$ is  strictly nef.
By induction (and {\hyperref[remark_conclude_excep_tocurve]{Remark    \ref*{remark_conclude_excep_tocurve}}}), $K_{X'}+t_0D_{X'}$ is ample for any (fixed) $t_0\gg 1$.
But then, $K_X+t_0D_X=\varphi^*(K_{X'}+t_0D_{X'})+E$ is big; thus $K_X+uL_X=\frac{1}{1+t_0\nu}(K_X+t_0D_X)+(u-\frac{t_0}{t_0\nu+1})L_X$ is also big for  $u\gg 1$, a contradiction (cf.~{\hyperref[lem-not-big-some]{Lemma  \ref*{lem-not-big-some}}}). 
Hence, there is an irreducible curve $B'\in\overline{\textup{NE}}(X')$ such that $D_{X'}\cdot B'=0$.
By 
{\hyperref[lem_intersect_C_<-1]{Lemma \ref*{lem_intersect_C_<-1}}},
$K_{X'}\cdot B'<0$.
Since $D_{X'}$ is nef, by the cone theorem (cf.~\cite[Theorem 3.7]{KM98}), there exists a $K_{X'}$-negative extremal curve $\ell'$ such that $K_{X'}\cdot\ell'<0$ and $D_{X'}\cdot\ell'=0$. %, which completes the proof.
\end{proof}

\begin{lemme}\label{lem-sec-con-surface}
If $K_X+tL_X$ is not ample for any $t\gg 1$, then the contraction $\varphi':X'\to X''$ of $\mathbb{R}_{\geqslant  0}[\ell']$ in {\hyperref[lem_not_big_X']{Lemma \ref*{lem_not_big_X'}}} is birational.	
\end{lemme}

\begin{proof}
Suppose the contrary that $\dim X''\leqslant 2$.
By the cone theorem (cf.~\cite[Theorem 3.7]{KM98}), $D_{X'}=\varphi'^*(D_{X''})$ for some nef divisor $D_{X''}$ on $X''$.
If $X''$ is a point, then $\rho(X')=1$ and $D_{X'}$ is ample, a contradiction to {\hyperref[prop-q-effective]{Proposition  \ref*{prop-q-effective}}}.
If $X''$ is a curve or  $\dim X''=2$ and $D_{X''}^2\neq 0$ (and hence big),
then $D_{X'}$ (and hence $D_X$) is numerically equivalent to a non-zero effective divisor, contradicting  {\hyperref[prop-q-effective]{Proposition  \ref*{prop-q-effective}}} again.

Suppose that $\dim X''=2$ and $D_{X''}^2=0$. 
We claim that the composite $\varphi'\circ\varphi:X\to X''$ is an equi-dimensional $K_X$-negative contraction (of an extremal face); thus we get a contradiction to our assumption by {\hyperref[thm_contr_surface_conic]{Theorem    \ref*{thm_contr_surface_conic}}}. 
First, by the cone theorem (cf.~\cite[Theorem 3.7]{KM98}), $\varphi$ is equi-dimensional (of relative dimension one).
Since $C'$ is not contracted by $\varphi'$ (cf.~{\hyperref[lem_D.C>0]{Lemma \ref*{lem_D.C>0}}}), the composite $\varphi'\circ\varphi$ is also equi-dimensional. 
Take any irreducible curve $F$ contracted by $\varphi'\circ\varphi$.
Then $D_X\cdot F=(\varphi'\circ\varphi)^*(D_{X''})\cdot F=0$ and thus $K_X\cdot F<0$.
Hence, $-K_X$ is $(\varphi'\circ\varphi)$-ample  (cf.~\cite[Theorem 1.42]{KM98}) and 
$\varphi'\circ\varphi$ is a $K_X$-negative contraction.
Finally, the contraction $X\to X''$ is  clearly extremal by 
considering the pullback of any ample divisor on $X''$. % to $X$.	
\end{proof}

The following lemma is a bit technical. 
We divide the proof into several cases for readers' convenience. 
We shall heavily apply the terminalization and {\hyperref[lem_canonical_terminal]{Lemma  \ref*{lem_canonical_terminal}}}.
Recall that the \textit{length} of a $K_X$-negative extremal contraction is defined to be the minimum of $-K_X\cdot B$ for generic curves $B$ in the covering families of contracted locus.

\begin{lemme}\label{lem_bir-intersectC}
If $K_X+tL_X$ is not ample for any $t\gg 1$, then the contraction $\varphi':X'\to X''$ of $\mathbb{R}_{\geqslant  0}[\ell']$ in {\hyperref[lem_not_big_X']{Lemma \ref*{lem_not_big_X'}}} is  divisorial  with the exceptional divisor  $E'$ such that   $E'\cap C'=\emptyset$.
\end{lemme}

\begin{proof}
%We may assume that $K_X+tL_X$ is not ample for any $t\gg 1$. 
By {\hyperref[lem-sec-con-surface]{Lemma  \ref*{lem-sec-con-surface}}}  and {\hyperref[lem_del14]{Lemma  \ref*{lem_del14}}},  our $\varphi'$ is  a divisorial contraction.
In the following, we shall discuss case-by-case in terms of $E'$ and the intersection of $E'\cap C'$.
\par \vskip 0.4pc \noindent
\textbf{Case (1). Suppose $C'\subseteq E'$.}  
Then $C'$ being rigid and $D_{X'}\cdot C'>0$ (cf.~{\hyperref[lem_L.C>0]{Lemma \ref*{lem_L.C>0}}} and {\hyperref[lem_D.C>0]{Lemma \ref*{lem_D.C>0}}}) would imply that $\varphi'$ is a blow-up of a curve on $X''$ (cf.~{\hyperref[lem_canonical_terminal]{Lemma  \ref*{lem_canonical_terminal}}}) with $C'$ being  horizontal  on $E'\subseteq X'$. 
Let $\ell'$ be a general fibre of $\varphi'$. 
Since $D_{X'}\cdot \ell'=0$ and $\ell' \cap C'\neq\emptyset$, we have $K_{X'}\cdot\ell'\leqslant -2$ (cf.~{\hyperref[lem_intersect_C_<-1]{Lemma \ref*{lem_intersect_C_<-1}}}),  contradicting {\hyperref[lem_del14]{Lemma  \ref*{lem_del14} (3)}}.

\par \vskip 0.4pc \noindent
\textbf{Case (2). Suppose  $E'\cap C'$ is a finite non-empty  set.} 
Then by {\hyperref[lem_canonical_terminal]{Lemma  \ref*{lem_canonical_terminal}}}, we have the following commutative diagram
\begin{align}\label{diagram_4}\tag{$*$}
\xymatrix{Y'\ar[r]^{\phi'}\ar[d]_{\tau'}&Y''\ar[d]^{\tau''}\\
X'\ar[r]_{\varphi'}&X''
}	
\end{align}
where $\tau'$ is the crepant terminalization, $\phi'$ is a divisorial contraction, and $Y'$ has only $\mathbb{Q}$-factorial Gorenstein terminal singularities.

\par \vskip 0.4pc \noindent
\textbf{(2i).} Suppose $\phi'$ maps the exceptional divisor $E_{Y'}$ to a point  and the length of  $\phi'$ is one (this is the case when \cite[Theorem 5 (2), (3) or (4)]{Cut88} happen). 
By {\hyperref[lem_canonical_terminal]{Lemma  \ref*{lem_canonical_terminal}}}, $E'\cong E_{Y'}$.  
Then we can pick a  
curve $\ell'\subseteq E'\subseteq X'$ of $\varphi'$ meeting $C'$ such that $K_{X'}\cdot\ell'=-1$ (noting that $\tau'$ is crepant) and $D_{X'}\cdot \ell'=0$. %(this is the case when Lemma \ref{lem_cut_surface_curve} or (2), (3), (4) of Lemma \ref{lem_cut_surface_point} happen); cf. \cite[Theorem 1.2]{Del14}.  
%Since $\ell'$ intersects with $C$ and $E$ is Cartier (cf.~Lemma \ref{lem_canonical_terminal}),  
 %$\hat{\ell'}\cdot E\geqslant 1$. %$$\varphi^*(\ell')=\hat{\ell'}+a\ell$$
%with a positive integer $a=E\cdot\hat{\ell'}\geqslant 1$.
%Then the strict nefness of $L_X$ and the following inequality
%$$K_X\cdot\hat{\ell'}=(\varphi^*K_{X'}+E)\cdot\hat{\ell'}=-1+\hat{\ell'}\cdot E\geqslant 0$$
%implies that $0=D_{X'}\cdot\ell'=D_X\cdot\hat{\ell'}=(L_X+\nu K_X)\cdot\hat{\ell'}>0$, a contradiction. 
However, this contradicts 
{\hyperref[lem_intersect_C_<-1]{Lemma \ref*{lem_intersect_C_<-1}}}.

\par \vskip 0.4pc \noindent 
\textbf{(2ii).} Suppose  $\phi'$ maps the exceptional divisor $E_{Y'}$ onto a curve   (and hence the length of  $\phi'$ is still one, which is the case when \cite[Theorem 4]{Cut88} happens).
Let $P\in E'\cap C'$.
If $P$ is a terminal point, then we 
pick a fibre $\ell_{Y'}\subseteq E_{Y'}$ passing through $\tau'^{-1}(P)$.
If $P$ is not a terminal point, then we take a curve $c_0\subseteq \tau'^{-1}(P)\cap E_{Y'}$, which is a horizontal curve of $\phi'$; in this case, we pick $\ell_{Y'}$ to be any fibre of $\phi'$, which automatically intersects with $c_0$.
In both cases, let $\ell':=\tau'(\ell_{Y'})\ni P$.  
Similarly, $K_{X'}\cdot\ell'=\tau'^*K_{X'}\cdot \ell_{Y'}=K_{Y'}\cdot \ell_{Y'}=-1$, which contradicts 
{\hyperref[lem_intersect_C_<-1]{Lemma \ref*{lem_intersect_C_<-1}}} again.
%https://www.imsc.res.in/xmlui/bitstream/handle/123456789/454/HBNI%20Th166.pdf?sequence=1&isAllowed=y 2.1.4

\par \vskip 0.4pc \noindent
\textbf{(2iii).} By the classification, we may assume that $\phi'$ maps the exceptional divisor $E_{Y'}$ to a point and the length of $\phi'$ is two (this is the case when \cite[Theorem 5 (1)]{Cut88} happens). 
In this case, $E_Y'\cong\mathbb{P}^2$ with $E_{Y'}|_{E_{Y'}}=\mathcal{O}(-1)$, $Y''$ (and hence $Y'$) is  smooth, and $\varphi'(E')$ is a point. 
Consider the following  (by taking $\tau_2:=\tau'$ and $\tau_3:=\tau''$ in the diagram (\ref{diagram_4})):
\begin{align}\label{diagram_5}\tag{$**$}
\xymatrix{Z\ar[d]_{\tau_0}&Y\ar[r]^{\phi}\ar[l]_{\psi_Y}\ar[d]_{\tau_1}&Y'\ar[r]^{\phi'}\ar[d]^{\tau_2}&Y''\ar[d]^{\tau_3}\\
W&X\ar[l]^{\psi_X}\ar[r]_\varphi &X'\ar[r]_{\varphi'}&X''
}	
\end{align}

\textbf{We first explain in the following how to get the  diagram (\ref{diagram_5}).}
By {\hyperref[lem_canonical_terminal]{Lemma  \ref*{lem_canonical_terminal}}}, we get the diagrams $\tau_2\circ\phi=\varphi\circ\tau_1$ and $\tau_3\circ\phi'=\varphi'\circ\tau_2$,
noting that $\textup{Exc}(\tau_1)$ is disjoint with $E_Y:=\textup{Exc}(\phi)$ and $\textup{Exc}(\tau_2)$ is  disjoint with $E_{Y'}:=\textup{Exc}(\phi')$.
This implies that $E'\cong E_{Y'}=\mathbb{P}^2$ and  $X'$ is smooth around $E'$.
Fixing a line $\ell'\subseteq E'$ of $\varphi'$ meeting $C'$ and taking $\hat{\ell'}$ to be its proper transform on  $X$,  we have
$K_{X'}\cdot \ell'=-2$.
Let $a:=\hat{\ell'}\cdot E\geqslant 1$. 
Then $K_X\cdot\hat{\ell'}=-2+a$ and $L_X\cdot\hat{\ell'}=\nu(2-a)>0$.
In particular, $a=1$ and $K_X\cdot\hat{\ell'}=-1$.
\textbf{This also implies that $E'$  meets $C'$ along a  single (smooth) point of $C'$.}
Indeed, if $\sharp (E'\cap C')\geqslant 2$, then the line $\ell'\subseteq E'$ passing through any two points of $E'\cap C'$ satisfies $E\cdot\hat{\ell'}\geqslant 2$, which is absurd. 
So the $\varphi$-proper transform $\hat{E'}\cong\mathbb{F}_1$ of $E'$ is ruled over $h_W\cong\mathbb{P}^1$ with fibres $\hat{\ell'}$ and the negative section $C_0$ (being a fibre of $\varphi$). 
Suppose $P\in E'\cap C'$ is a singular point  of $C'$.  
Then   $E'\cdot C'=\deg \mathcal{O}_{X'}(E')|_{\widetilde{C'}}\geqslant 2$, with $\widetilde{C'}$  the normalization of $C'$, in which case,
any line $\ell'\subseteq E'$ containing $P$ satisfies  $E\cdot\hat{\ell'}=(E|_{\hat{E'}}\cdot\hat{\ell'})_{\hat{E'}}=(C'\cdot E')\geqslant 2$, a contradiction.
So  $E'$ meets $C'$ along a single smooth point of $C'$.
%otherwise $E'\cdot C'=\deg E'|_{normalization of C'}\geqslant 2$, and thus $E\cdot\hat{\ell'}=(E|_{\varphi^*E'}\cdot\hat{\ell'})_{\varphi^*E'}=\varphi^{-1}((C'\cdot E')p)\cdot\hat{\ell'}$.
%Note that $E'$ can meet $C$ only along a single point (transversely). 
%Otherwise, there exists a line $B\subseteq E'$ passing through two points of $E'\cap C$.
%Then the strict transform $\hat{B}\subseteq X$ satisfies $E\cdot\hat{B}\geqslant 2$ and hence $K_X\cdot\hat{B}=K_{X'}\cdot B+E\cdot\hat{B}\geqslant 0$, contradicting Lemma \ref{lem_intersect_C_<-1}. 
%Since ,
%our $X$ is smooth around $\hat{E'}$.

Since $\hat{E'}\cdot\hat{\ell'}=\varphi^*E'\cdot\hat{\ell'}=-1$ (noting that $E'|_{E'}=\mathcal{O}(-1)$) and  $-\hat{E'}|_{\hat{E'}}$ is  relative ample with respect to the ruling $\hat{E'}\to h_W$, we obtain a contraction $\psi_X:X\to W$   such that $\psi_X|_{\hat{E'}}$ coincides with this ruling and $\psi_X|_{X\backslash\hat{E'}}\cong W\backslash h_W$ (cf.~e.g.~\cite[Proposition 7.4]{HP16}). 
Similar to $\psi_X$, the morphism $\psi_Y$ is induced by contracting the divisor $\hat{E}_{Y'}:=\tau_1^*\hat{E'}\cong\mathbb{F}_1$ to $h_Z\cong h_W\cong\mathbb{P}^1$. 
By the rigidity lemma, $\psi_X\circ\tau_1$ factors through $\psi_Y$ 
and we get $\tau_0$.

\textbf{Caution: it is still not clear whether $W$ is projective or not, and  $\psi_X$ here may not be an extremal contraction.
Therefore, we could not apply the induction on $W$ so far.} 

Since $X$ has only canonical singularities and $L_X+\nu\hat{E'}$ is $\psi_X$-trivial,  
by \cite[Theorem 4.12]{Nak87}, there exists a  divisor  $L_W$ on $W$ such that
$L_X=\psi_X^*(L_W)-\nu\hat{E'}$. 
Recall that $C_0$ (a fibre of $\varphi$) is the negative section of $\hat{E}'$. %(which is contracted by $\varphi$). 
Since $-{\hat{E'}}|_{{\hat{E'}}}=C_0+\hat{\ell'}$ (noting that $\hat{E'}\cdot\hat{\ell'}=E'\cdot\ell'=-1$ and $\hat{E'}\cdot C_0=0$), we obtain the following strictly nef divisor on $\hat{E'}$
$$L_X|_{\hat{E}'}=\nu C_0+(L_W\cdot h_W+\nu)\hat{\ell'}.$$
Since  a strictly nef divisor on $\mathbb{F}_1$ is ample, our $L_X|_{\hat{E}'}$ is ample and hence  $L_W\cdot h_W>0$ (cf.~\cite[Chapter 5, Proposition 2.20]{Har77}). 
Then $L_W$ is strictly nef on the Moishezon threefold $W$ by the projection formula. 
We consider the following commutative diagram:
\[\xymatrix{
Z_0\ar[d]_{\sigma_0}\ar@/_2pc/[dd]_{\pi_0}&Y_0\ar[l]_{\psi_{Y_0}}\ar[d]^{\sigma_1}\ar@/^2pc/[dd]^{\pi_1}\\
Z\ar[d]_{\tau_0}&Y\ar[d]^{\tau_1}\ar[l]_{\psi_Y}\\
W&X\ar[l]^{\psi_X}
}
\]
where $\sigma_1:Y_0\to Y$ is a resolution with $Y_0$ being smooth.
Since $X$ is smooth around $\hat{E'}$ (recalling that $E'\cap C'$  is a smooth point of $C'\subseteq X'$), our $Y$ is also smooth around $\hat{E}_{Y'}$.
So  $\sigma_1$ is isomorphic around $\hat{E}_{Y'}$.
In particular, $Y_0$ admits a contraction $\psi_{Y_0}$ mapping $E_{Y_0}:=\sigma_1^*(\hat{E}_{Y'})=\pi_1^*\hat{E'}\cong\mathbb{F}_1$ onto a curve $h_{Z_0}\cong\mathbb{P}^1$ (cf.~e.g. \cite[Proposition 7.4]{HP16}).
By the rigidity lemma, $\psi_Y\circ\sigma_1$ factors through $\psi_{Y_0}$, and we get the induced $\sigma_0$.
Since  $Y_0$ is smooth and the conormal sheaf of $E_{Y_0}$ is isomorphic to $-E_{Y_0}|_{E_{Y_0}}$ which is (locally over $h_{Z_0}$) isomorphic to $\mathcal{O}(1)$, 
it follows from \cite[Corollary 6.11]{Art70} that $Z_0$ is smooth.
\begin{claim}\label{claim_proj}
$Z_0$ is projective.	
\end{claim}

Suppose the claim for the time being. 
Since $-K_X$ is $\psi_X$-ample, we have $R^j(\psi_X)_*\mathcal{O}_X=0$ for all $j\geqslant 1$ (cf.~\cite[Theorem 1-2-5]{KMM87}) and  hence $W$ has only isolated rational singularities.
Since $Z_0\to W$ is a resolution and $Z_0$ is projective by the assumption, 
by \cite[Remark 3.5]{HP16}, $W$ admits a (smooth) K\"ahler form and hence $W$ is both K\"ahler and Moishezon.
So the projectivity of $W$ follows from \cite[Theorem 6]{Nam02}.
Now, $W$ being projective and $L_W$ being strictly nef, we get a contradiction by (Proof of) {\hyperref[lem_L.C>0]{Lemma \ref*{lem_L.C>0}}}.

\par \vskip 1pc \noindent
\textbf{Proof of {\hyperref[claim_proj]{Claim \ref*{claim_proj}}}  (End of Proof of {\hyperref[lem_bir-intersectC]{Lemma \ref*{lem_bir-intersectC}}}).}
Suppose the contrary. 
Denote by $\pi_i:=\tau_i\circ\sigma_i$.
By  \cite[Theorem 2.5]{Pet86}, there is an irreducible curve $b$ and a positive closed current $T$ on $Z_0$ such that $b+T\equiv0$ (as $(2,2)$-currents); hence $(\pi_0)_*(b+T)\equiv0$.
Since $L_W$ is strictly nef on $W$, our $b$ is $\pi_0$-exceptional.
Note that $X$ is smooth around $\hat{E'}$ and $\hat{E}_{Y'}\cap \textup{Exc}(\tau_1)=\emptyset$.
So $E_{Y_0}\cap\textup{Exc}(\pi_1)=\emptyset$.
Take a very ample divisor $H$ on $Y_0$.
Since $Z_0$ is $\mathbb{Q}$-factorial, it is easy to verify that $(\psi_{Y_0})_*H\cdot b>0$ (cf.~\cite[Lemma 2.62]{KM98}), noting that $\pi_0^*L_W\cdot h_{Z_0}>0$   and thus $b\neq h_{Z_0}:=\psi_{Y_0}(E_{Y_0})$.
%Indeed, for any curve $b\neq h_Z$, we have $(\psi_Y)_*H\cdot b>0$.
So  $(\psi_{Y_0})_*H\cdot T<0$.
By \cite{Siu74}, our $T=\chi_{h_{Z_0}}T+\chi_{Z_0\backslash h_{Z_0}}T=\delta h_{Z_0}+\chi_{Z_0\backslash h_{Z_0}}T$, where $\chi_{h_{Z_0}}T$ and $\chi_{Z_0\backslash h_{Z_0}}T$ are positive closed currents. 
Since $(\psi_{Y_0})_*H\cdot \chi_{Z_0\backslash h_{Z_0}}T\geqslant 0$, we have $\delta>0$.
Then
$$0\equiv (\pi_0)_*(b+T)\equiv (\pi_0)_*T=\delta h_W+(\pi_0)_*(\chi_{Z_0\backslash h_{Z_0}}T).$$
 Since $L_W\cdot h_W>0$ and $L_W\cdot(\pi_0)_*(\chi_{Z_0\backslash h_{Z_0}}T)\geqslant 0$, the above equality is absurd.
\end{proof}

\begin{proof}[\textup{\textbf{End of Proof of {\hyperref[thm_3fold_surface_curve]{Theorem \ref*{thm_3fold_surface_curve}}}.}}]
We suppose the contrary that $K_X+tL_X$ is not ample for any $t\gg 1$. 
By {\hyperref[lem-sec-con-surface]{Lemma \ref*{lem-sec-con-surface}}}
 and {\hyperref[lem_bir-intersectC]{Lemma \ref*{lem_bir-intersectC}}}, 
 $\varphi':X'\to X''$ is a divisorial contraction with the exceptional divisor $E'$  disjoint with $C'$.
Then the strict transform of $E'$ on $X$ is some $E_j$, $j\in I_0$ (cf.~{\hyperref[not_bir_surface_curve]{Notation  \ref*{not_bir_surface_curve}}}); hence we can continue to consider $D_{X''}$.
%We may further assume $D_{X''}$ is not big but strictly nef on $X''$. 
By {\hyperref[prop-q-effective]{Proposition  \ref*{prop-q-effective}}} and the induction  on $X''$ (cf.~{\hyperref[remark_conclude_excep_tocurve]{Remark    \ref*{remark_conclude_excep_tocurve}}}),  our $D_{X''}$ is  not strictly nef. 
So we get the third  contraction $X''\to X'''$ (cf.~{\hyperref[lem_not_big_X']{Lemma \ref*{lem_not_big_X'}}}). 
If $\dim X'''\leqslant 2$, then we  argue as in {\hyperref[lem-sec-con-surface]{Lemma \ref*{lem-sec-con-surface}}}, together with {\hyperref[thm_contr_surface_conic]{Theorem    \ref*{thm_contr_surface_conic}}}, to conclude that $K_X+tL_X$ is ample, a contradiction to our assumption.   
So $X''\to X'''$ is still birational with the exceptional divisor $E''$. 
But then, {\hyperref[lem_bir-intersectC]{Lemma \ref*{lem_bir-intersectC}}} Case (1) shows that neither $\varphi'(C')$ (where $C'=\varphi(E)\subseteq X'$) nor $C''$ (where $C''=\varphi'(E')\subseteq X''$) is contained in $E''$.
Further,  {\hyperref[lem_bir-intersectC]{Lemma \ref*{lem_bir-intersectC}}} Case (2) gives that
 such $E''$ cannot intersect with  $\varphi'(C')\cup C''$. %; indeed, if   Lemma \ref{lem_bir-intersectC} Case (2iii) happens, one can similarly show that such $E''$ cannot intersect with  $\varphi'(C')$ and $C''$ at the same time (for otherwise, there is a line in $E''\cong\mathbb{P}^2$ connecting such two intersection points). 
Hence,  $E$, $E'$ and $E''$ are pairwise disjoint. 
Since  $X$ is uniruled, after finitely many steps, we get some $X_M$ with $\dim X_M\leqslant 2$. 
By {\hyperref[thm_contr_surface_conic]{Theorem    \ref*{thm_contr_surface_conic}}}, $K_X+tL_X$ is ample which contradicts our assumption (cf.~{\hyperref[lem-sec-con-surface]{Lemma \ref*{lem-sec-con-surface}}}).
\end{proof}

\begin{proof}[Proof of {\hyperref[main_theorem_Goren_ter_3fold]{Theorem   \ref*{main_theorem_Goren_ter_3fold} (3)}}]
It follows  from {\hyperref[remark_conclude_excep_tocurve]{Remark    \ref*{remark_conclude_excep_tocurve}}} and 	{\hyperref[thm_3fold_surface_curve]{Theorem \ref*{thm_3fold_surface_curve}}}.
\end{proof}

%\end{appendices}
